# Supplementary material for: Methods for Population Adjustment with Limited Access to Individual Patient Data: A Review and Simulation Study
Source: arXiv:2004.14800 ancillary file (2021-06-02)
Supplement: Supplementary file 1 [file population_adjustment_supplementary_material.pdf]

# Supplementary Material of Methods for Population Adjustment with Limited Access to Individual Patient Data: A Review and Simulation Study

Antonio Remiro-Azócar, Anna Heath, Gianluca Baio

## Appendix A: Method assumptions

In practice, we consider that a causal treatment effect is of interest in any indirect comparison between treatments, which ultimately seeks to mimic the analysis that would be conducted in a head-to-head RCT. This discussion of assumptions borrows terminology from the potential outcomes framework for causal inference, commonly known as the Rubin Causal Model (Holland 1986), originally proposed by Neyman (1923) in the analysis of randomized experiments, and generalized to observational studies by Rubin (1974). We introduce the assumptions made by population-adjusted indirect comparisons in this context. Note that this discussion is non-technical and detailed theory and notation based on potential outcomes is not presented.

Population-adjusted indirect comparisons make the following assumptions, required to make valid causal inferences: (1) internal validity; (2) consistency under parallel studies; (3) conditional strong ignorability of trial assignment for the  $A$  vs.  $C$  treatment effect (this requires both the conditional constancy of relative effects and overlap/positivity across the covariate distributions); (4) correct specification of the  $BC$  population; and (5) linear modeling assumptions. The first two assumptions are shared by MAIC, STC and the Bucher method; in fact, these are made by any indirect comparison or meta-analysis. Assumptions that are not specific to indirect treatment comparisons, e.g. related to measurement error or missing data, or that are specific to the type of regression model used, e.g. proportional hazards or non-informative censoring for a Cox regression, are not discussed.

Note that the following assumptions can only guarantee an unbiased comparison if the within-trial relative effects target compatible estimands of the same type. The majority of RCTs publish an estimate for  $B$  vs.  $C$  that targets a marginal treatment effect (any published estimate of a conditional treatment effect is likely incompatible with that for  $A$  vs.  $C$  if the measure of effect is non-collapsible). Hence,  $\hat{\Delta}_{AC}$  (for the Bucher method) or  $\hat{\Delta}_{AC}^*$  (for the population adjustment methods) should target a marginal treatment effect. If a comparison of conditional treatment effects is performed, these would have to be adjusted across identical sets of covariates, using the same model specification.

In the case of an unanchored comparison, some consider that causal conclusions cannot be obtained based on non-randomized data alone. A causal interpretation of the treatment effect can be supported by the framework outlined in this appendix, but the assumptions required are somewhat heroic.

It is worth noting that, throughout the text, when referring to the  $AC$  and  $BC$  “populations”, we are in fact referring to the  $AC$  and  $BC$  study samples. In other contexts, these are viewed as samples of the populations, which in turn are defined by the inclusion/exclusion criteria of the trials. In our context, the trial samples represent the populations, i.e., one assumes that the sampling variability in their descriptive characteristics is ignored.

In addition, it is worth noting that when referring to “effect modifiers”, we refer to the variables that modify the treatment effect measure for  $A$  vs.  $C$  in the linear predictor scale. We select the effect modifiers of treatment  $A$  with respect to  $C$  (as opposed to the effect modifiers of treatment  $B$  with respect to  $C$ ), because we have to adjust for these to perform the indirect comparison in the  $BC$  population, implicitly assumed to be the target population. If we had IPD for the  $BC$  study and ALD for the  $AC$  study, we would have to account for the covariates that modify the effect of treatment  $B$  vs.  $C$ , in order to perform the comparison in the  $AC$  population.

## Internal validity

The first set of assumptions relates to the internal validity of the *AC* and *BC* trials. The trials are internally valid under the following structural assumptions, which are necessary for causal inference:

- Stable unit treatment value assignment (SUTVA). This assumption implies that: (1) the treatment of a given subject does not affect the potential outcomes of other individuals (non-interference) (Rubin 1980); and (2) there is only one version of each treatment (treatment-variation irrelevance) (VanderWeele 2009), implying that the treatment is comparable across units (VanderWeele and Hernan 2013).
- Strongly ignorable treatment assignment. Ignorability implies that treatment assignment is independent of the potential outcomes conditional on the observed baseline characteristics (Rosenbaum and Rubin 1983), regardless of whether these are prognostic variables or effect modifiers. Ignorability is strong when there is positivity (Hernán and Robins 2006) or overlap, i.e., any subject has a positive probability of being assigned to either treatment group given the baseline covariates.

The SUTVA assumption is met by appropriate study design (Rubin 2005). By design, the conditions of positivity (Cole and Hernán 2008) and ignorability (Greenland and Robins 2009) are met by randomized trials. The random allocation of treatment ensures that, on expectation, there are no systematic differences in the distribution of baseline covariates between treatment groups, i.e., there is covariate balance (Austin 2013). Note that balance is a large sample property. In small samples, one may still observe residual differences in baseline characteristics that bias the comparison. Therefore, the internal validity assumptions are met if the *AC* and *BC* trials are appropriately designed studies with proper randomization and reasonably large sample sizes. Internal validity is sufficient for unbiased estimation of  $\Delta_{AC}$  and  $\Delta_{BC}$  within each trial.

**Unanchored comparison.** In the unanchored case with single-arm studies, strongly ignorable treatment assignment is not required as there is no common comparator arm. However, unanchored comparisons are subject to the additional assumptions and biases of non-randomized study designs, which are often stronger (Deeks et al. 2003).

## Consistency under parallel studies

Consistency under parallel studies (Hartman et al. 2015) is the cross-trial version of the second condition of SUTVA (treatment-variation irrelevance). This assumption implies that potential outcomes for an individual under a given treatment are homogeneous regardless of the study assigned to the individual. For instance, treatment *C* should be administered in the same setting in both trials, or differences in the nature of treatment, e.g. in the clinical protocol, should not change its effect.

Consistency under parallel studies means that MAIC and STC cannot adjust for cross-trial differences related to the nature of treatments, e.g. treatment administration, switching, dosing formulation, titration or co-treatments. Differences of this type are perfectly confounded with treatment (Phillippo et al. 2016), and MAIC and STC can only adjust for differences in trial population characteristics. This assumption is required to perform any valid indirect comparison across studies.

## Conditionally strong ignorability of trial assignment

Strongly ignorable trial assignment (specifically, assignment to the *AC* trial), is the primary assumption underlying population-adjusted indirect comparisons and is required for unbiased estimation of  $\Delta_{AC}^*$ . This is akin to the strongly ignorable sample assignment assumption (Hartman et al. 2015) commonly used in the generalizability literature (Hartman et al. 2015; Cole and Stuart 2010; Stuart et al. 2011; Kern et al. 2016). Generalizability seeks to extend relative treatment effects obtained from a RCT into a target population — the trial sample is considered to be an unrepresentative subpopulation of the, more diverse, target population. In MAIC and STC, the indirect comparison is performed in the *BC* population, and the *A* vs. *C* treatment effect is “generalized” to the *BC* population. Strong ignorability collectively relies on two assumptions: ignorability and overlap (or positivity). Note that, even though strong ignorability has been proposed in the context of propensity score modeling, it is also required for robust inference when using regression adjustment approaches to estimate treatment effects.

## Conditional ignorability

This assumption has many possible formulations. In the anchored case, one can consider that trial assignment/selection is conditionally ignorable, unconfounded or exchangeable for the  $A$  vs.  $C$  treatment effect (the potential relative outcomes for  $A$  vs.  $C$ ), i.e., being in study  $AC$  or study  $BC$  does not carry over any information about such treatment effect, once we condition on the treatment effect modifiers. This means that after accounting for these effect modifiers, treatment effect heterogeneity and trial assignment are conditionally independent.

MAIC will only meet conditional ignorability if *all* (observed or unobserved) effect modifiers are accounted for, regardless of whether these are balanced before the weighting (excluding balanced covariates from the weighting procedure does not ensure balance after the weighting). STC meets conditional ignorability if all *imbalanced* effect modifiers are accounted for in the regression model.

This assumption is challenging to meet in practice and also untestable. On one hand, it is tied to the scale used to define the treatment effects and effect modifiers. Most importantly, it requires that all effect modifiers are measured in the IPD for study  $AC$  and that the set of published baseline characteristics for study  $BC$  is sufficiently rich, such that all effect modifiers are available. This is a key challenge as “Table 1” data on the published RCT for the  $BC$  population are often limited, and it can sometimes be difficult to find common measures between different studies. In addition, all effect modifiers must be accounted for by the analyst, who may select the effect modifiers incorrectly. It is generally difficult to ascertain the effect modifier status of variables, particularly for new treatments with limited prior empirical evidence and clinical domain knowledge. Overspecification of effect modifiers will not bias the comparison but may inflate standard errors and lead to a subsequent loss of precision.

**Unanchored comparison.** In this case, trial assignment is ignorable if it is conditionally independent of the potential absolute outcomes given the effect modifiers and prognostic variables accounted for in the adjustment mechanism. MAIC and STC only meet ignorability if all (observed or unobserved) effect modifiers and prognostic variables are balanced. This requires complete information on all treatment effect modifiers and prognostic variables to be measured across trials, and for all of these to be accounted for by the analyst. In the unanchored case, ignorable trial assignment is equivalent to the conditional constancy of absolute effects described in the literature (Phillippo et al. 2016, 2018).

## Overlap

Conditional ignorability of trial assignment is strong if there is positivity or overlap, i.e., if every subject in the  $BC$  population has a positive probability of being assigned to the  $AC$  trial given the effect modifiers. This implies that the ranges of the effect modifiers in the  $BC$  population are covered by their respective ranges in the  $AC$  trial. This assumption may pose a problem if the inclusion/exclusion criteria of  $AC$  and  $BC$  are inconsistent. For instance, consider a situation where age is an effect modifier and the age ranges of trial  $AC$  and trial  $BC$  are 60-70 and 40-70, respectively. There exists a subpopulation (age 40-60) in  $BC$  that does not overlap with the  $AC$  population. Hence, the  $AC$  study provides no evidence or information about the treatment effect and treatment effect modification in the excluded age group, and  $\hat{\Delta}_{AC}^*$  may be biased in the full comparator trial population (ages 40-70).

In such cases, weighting methods like MAIC are unable to extrapolate beyond the observed covariate space in the  $AC$  IPD, as there are no subjects to reweight. Where overlap is insufficient, a regression adjustment method like STC can extrapolate beyond the  $AC$  population, using the linearity assumption or other appropriate assumptions about the input space. However, valid extrapolation requires accurately capturing the true relationship between the effect modifiers and the outcome.

Conversely, the exclusion of patients enrolled in  $AC$  from the  $BC$  population, e.g. if the  $AC$  population is more diverse, does not necessarily violate the overlap assumption in MAIC and STC. This is because these methods deliver estimates in the  $BC$  population. Therefore, adjustment in this scenario is an interpolation as opposed to an extrapolation of the observed subject-level data for  $AC$ . In this scenario,  $\hat{\Delta}_{AC}^*$  may be unbiased because the  $BC$  population is covered within that of  $AC$ . In MAIC, the excluded subpopulation will receive very low weights (low odds of enrolment in  $BC$  vs.  $AC$ ), while the included subpopulation receives high weights and dominates the reweighted sample. These extreme weights lead to large reductions in ESS and to the deterioration of precision and efficiency. Removing observations from the  $AC$  patient-level data, so that inclusion/exclusion criteria are consistent, explicitly lowers the  $AC$  sample size and may degrade precision further. Of course, when there is no interpolation or extrapolation overlap whatsoever, MAIC cannot generate a population-adjusted estimate for the treatment effect.

**Unanchored comparison.** Ignorability of trial assignment is strong if there is positivity or overlap, i.e., if every subject in the *BC* population has a positive probability of being assigned to the *AC* trial given the effect modifiers and the prognostic variables. This implies that the ranges of the effect modifiers and of the prognostic variables in the *BC* population are covered by their respective ranges in the *AC* trial.

## Correct specification of the *BC* population

MAIC and STC make certain assumptions about the joint distribution of covariates in the *BC* trial. The restriction of limited IPD makes it unlikely that such joint distribution is available. Summary statistics for the marginal distributions are typically published instead.

In MAIC, as stated in the NICE Decision Support Unit Technical Support Document (Phillippo et al. 2016), “when covariate correlations are not available from the (*BC*) population, and therefore cannot be balanced by inclusion in the weighting model, they are assumed to be equal to the correlations amongst covariates in the pseudo-population formed by weighting the (*AC*) population.” In the typical usage of STC (i.e., the “plug-in” approach to the method), the assumption differs slightly. It is implicitly assumed that the joint distribution of the *BC* covariates is the product of the published marginal distributions. In the “covariate simulation” approach to STC, the assumption is more explicit: it is assumed that correlations between the *BC* covariates equal those observed in the *AC* IPD. In an anchored comparison, only effect-modifying covariates need balancing, so the assumption can be relaxed to only include effect modifiers. This set of assumptions only induces bias if second or higher order interactions with treatment (e.g. the three-way interaction of two effect modifiers and treatment) are misspecified.

**Unanchored comparison.** In the unanchored case, both effect modifiers and prognostic variables need balancing; hence the assumption must include them both.

## Linear modeling assumptions

Indirect treatment comparisons should be performed and are typically conducted on the linear predictor scale (Phillippo et al. 2016), upon which treatment is assumed to be additive for all indirect comparisons. MAIC and STC additionally assume that the effect modifiers have been defined on the linear predictor scale and are additive on this scale, but this assumption is not always appropriate.

MAIC and STC are subject to scale conflicts or to bias when treatment effect modification is non-linear or multiplicative. This form of model misspecification is more evident in a regression adjustment method like STC, where an explicit outcome regression is formulated. The parametric model depends on functional form assumptions that will be violated if the relationship between the effect modifiers and the outcome is not captured correctly, in which case STC may be biased.

Note that MAIC is also susceptible to bias in a more implicit form, as the logistic regression model for trial selection imposes a functional form on effect modification — effect modifiers are assumed to be additive on the linear predictor scale. The logistic regression model for the weights will be incorrectly specified if this is not the case, potentially leading to biased estimates in the indirect comparison.

Scale conflicts may also arise if effect modification status, which is scale-specific, has been justified on a different scale than that of the indirect comparison, e.g. on the natural outcome scale as opposed to the linear predictor scale.

**Unanchored comparison.** In the unanchored case, MAIC and STC also assume that the prognostic variables are additive on the linear predictor scale. Unanchored comparisons will also be subject to bias when the prognostic variables have a non-linear or multiplicative relationship with outcome, e.g. age in cardiovascular disease.

## Shared effect modification

MAIC and STC only produce an estimate  $\hat{\Delta}_{AB}^*$  that is valid in the *BC* population, implicitly assumed to be the target population. This may not match the target population for the decision, unless an additional assumption is made: the shared effect modifier assumption (Phillippo et al. 2016). Otherwise, one must assume that the target population of the comparison is the *BC* population.

This assumption is untestable with the available data and implies that: (1) active treatments  $A$  and  $B$  have the same set of treatment effect modifiers; and (2) the interaction effects of each effect modifier are identical for both treatments. Then, estimate  $\hat{\Delta}_{AB}^*$  can be transported to any given target population as effect modifiers are guaranteed to cancel out (relative effects for  $A$  vs.  $B$  are conditionally constant across all populations).

Shared effect modification is hard to meet in practice if the competing interventions do not belong to the same class, and have dissimilar mechanisms of action or clinical properties. In that case, there is little reason to believe that treatments  $A$  and  $B$  have the same set of effect-modifying covariates and that these interact with active treatment in the same way in  $AC$  and  $BC$ .

## Concluding remarks

In practice, some of the assumptions above may be hard to meet. Population-adjusted analyses require a larger number of assumptions than standard comparisons. These may be untestable with the available data, and will create additional complexity. Violations of the assumptions may lead to biased estimates of the treatment effect. Hence, it is important that future simulation studies assess the robustness of the methods to failures of the assumptions considered in this article, and under different degrees of data availability and model misspecification.

## Appendix B: Simulation study design

The simulation study is reported following the ADEMP (Aims, Data-generating mechanisms, Estimands, Methods, Performance measures) structure (Morris, White, and Crowther 2019). All simulations and analyses were performed using R software version 3.5.3 (Team and others 2013). The **survival** package (Therneau and Grambsch 2000) is used to perform standard (STC) and weighted (MAIC) Cox proportional hazards regressions. The files required to run the simulations are available at [https://github.com/remiroazocar/population\\_adjustment\\_simstudy](https://github.com/remiroazocar/population_adjustment_simstudy).

### Aims

We aim to compare MAIC, STC and the Bucher method in a wide range of scenarios, reflecting situations that may be encountered in practice, and to explore whether the methods are stretched to breaking point. The following properties are desirable for the methods:

1. **Unbiasedness** of the estimator in finite samples  $[E(\hat{\Delta}) = \Delta]$
2. **Variance unbiasedness**. The within-simulation standard error of  $\hat{\Delta}$  should be consistent with the average standard deviation across simulations.
3. **Randomization validity**. Coverage should be approximately equal to the nominal coverage rate, i.e., in a sufficiently large number of repetitions,  $(100 \times (1 - \alpha))\%$  confidence intervals based on normal distributions should contain the true value  $(100 \times (1 - \alpha))\%$  of the time, for a nominal significance level  $\alpha$ .
4. **Precision**. The true variance  $V(\hat{\Delta})$  of the estimator, estimated under a large number of simulations, should be as small as possible.

### Data-generating mechanisms

We consider survival or time-to-event outcomes in our simulation study, using the log hazard ratio as the measure of effect. We use the simulation procedure by Bender et al. (Bender, Augustin, and Blettner 2005) to generate Weibull-distributed survival times  $\tau_i$  for trials *AC* and *BC*. Four binary covariates are considered (two of these are purely prognostic variables and the other two are both effect modifiers and prognostic variables). Several factors are varied in a fully factorial arrangement with  $3 \times 3 \times 3 \times 3 \times 2 = 162$  scenarios. The values of the parameters and the rationale behind these is outlined below:

- The number of patients in the *AC* trial,  $N \in \{300, 450, 600\}$  under a 1:1 active intervention vs. control allocation ratio. The sample sizes correspond to typical values for a Phase III randomized controlled trial and for trials included in applications of MAIC and STC submitted to HTA authorities.
- The strength of the association between each prognostic variable  $k$  and the outcome,  $\beta_{1,k} \in \{-\log(0.67), -\log(0.5), -\log(0.33)\}$  (moderate, strong and very strong prognostic variable effect). These values correspond to fixing the conditional hazard ratios for the effect of each prognostic variable at approximately 1.5, 2 and approximately 3, respectively.
- The strength of effect-modifying interactions with treatment,  $\beta_{2,k} \in \{-\log(0.67), -\log(0.5), -\log(0.33)\}$  (moderate, strong and very strong interaction effect), where  $k$  indexes a given effect modifier. These parameters have a material impact on the *A* vs. *B* treatment effect. Population adjustment is warranted in order to remove the induced bias.
- The level of correlation between covariates,  $\text{cor}(X_{i,k}, X_{i,l}) \in \{0, 0.35\}$  (no correlation and moderate correlation), for subject  $i$  and covariates  $k \neq l$ .
- The degree of covariate imbalance. For both trials, each covariate  $k$  follows a normal marginal distribution. For the *BC* trial, we fix  $X_{i,k} \sim \text{Normal}(0.6, 0.2^2)$ , for subject  $i$ . For the *AC* trial, the normal distributions have mean  $\mu_k$ , such that  $X_{i,k} \sim \text{Normal}(\mu_k, 0.2^2)$ , varying  $\mu_k \in \{0.45, 0.3, 0.15\}$ . This yields strong, moderate and poor covariate overlap, respectively, corresponding to average percentage reductions in ESS across scenarios of 19%, 53% and 79%. These percentage reductions in ESS are representative of the range encountered in NICE TAs (see below).

## Further comments

As most applications of MAIC and STC are in oncology, the survival outcome may represent time to disease progression or death (progression-free survival) or time to death (overall survival). Each active intervention has a very strong conditional treatment effect at baseline (when the effect modifiers are zero) of  $\beta_T = \log(0.25)$  versus the common comparator.

We introduce random right censoring to simulate loss to follow-up within each trial. Censoring times  $\tau_{c,i}$  are generated from the exponential distribution  $\tau_{c,i} \sim \text{Exp}(\lambda_c)$ , where the rate parameter  $\lambda_c = 0.96$  is selected so that the expected censoring rate is 35% under the active treatment (when the prognostic variables and effect modifiers are zero), considered moderate censoring. We obtain the value of  $\lambda_c$  before generating the datasets by simulating survival times for 1,000,000 subjects and using the R function `optim` (Brent’s method) to minimize the difference between the observed and targeted censoring proportion. For each patient, we compare  $\tau_{c,i}$  with the latent survival time  $\tau_i$ : the time-to-event is censored at  $\tau_{c,i}$  if  $\tau_{c,i} < \tau_i$ ; otherwise, the event is observed at  $\tau_i$ .

The number of subjects in the *BC* trial is 600, under a 1:1 active treatment vs. control allocation ratio. Different values are not explored as these drive performance less than the number of subjects in the *AC* trial. While the number of subjects in *BC* contributes to sampling variability, the reweighting or regressions are performed in the *AC* patient-level data.

The prognostic variables and effect modifiers may represent comorbidities which are associated with lowered survival rates or which interact with treatment to render it less effective. Figure 1 shows the Weibull-distributed survival curves for patients under the active treatment (*A* and *B*) with varying levels of the covariates. Figure 2 shows the Weibull-distributed survival curves for subjects under the common comparator (*C*). The inverse scale is set to  $\lambda = 8.5$  and the shape to  $\nu = 1.3$  at baseline. In Figures 1 and 2, the strength of each prognostic term and each effect-modifying interaction is moderate. The varying degrees of covariate overlap are inspired by applications of MAIC in technology appraisals submitted to the National Institute for Health and Care Excellence. Only 13 of the 26 appraisals carrying out a MAIC have effective sample sizes available, albeit some appraisals contain multiple comparisons for different endpoints. In most applications, matching considerably reduces the effective sample size from the original *AC* sample size. The median percentage reduction is 58% (range: 7.9% to 94.1%; interquartile range: 42.2% to 74.2%).

Table 1 displays the average percentage reduction in effective sample size across different scenario settings. These are roughly representative of the range encountered in practice in NICE technology appraisals (Phillippo et al. 2019). The final effective sample sizes are also representative of those in the technology appraisals, which are also small (median: 80; range: 4.8 to 639; interquartile range: 37 to 174).

Table 1: Average effective sample size (ESS) percentage reduction across scenarios for matching-adjusted indirect comparison.

| Covariate overlap | Covariate correlation | Average percentage reduction in ESS |
|-------------------|-----------------------|-------------------------------------|
| Strong            | Moderate              | 16.3                                |
| Strong            | None                  | 21.0                                |
| Moderate          | Moderate              | 48.5                                |
| Moderate          | None                  | 58.4                                |
| Poor              | Moderate              | 75.1                                |
| Poor              | None                  | 83.5                                |

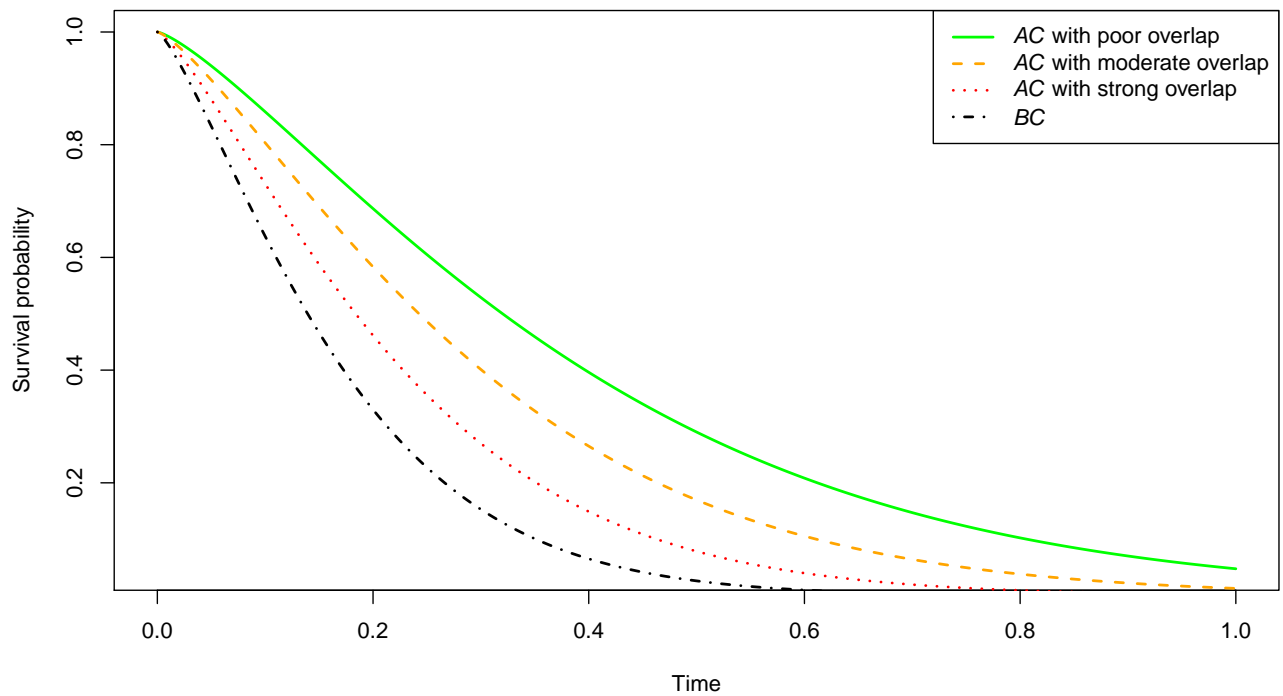

Figure 1: Weibull-distributed curves used to simulate survival times for subjects under the active treatment.

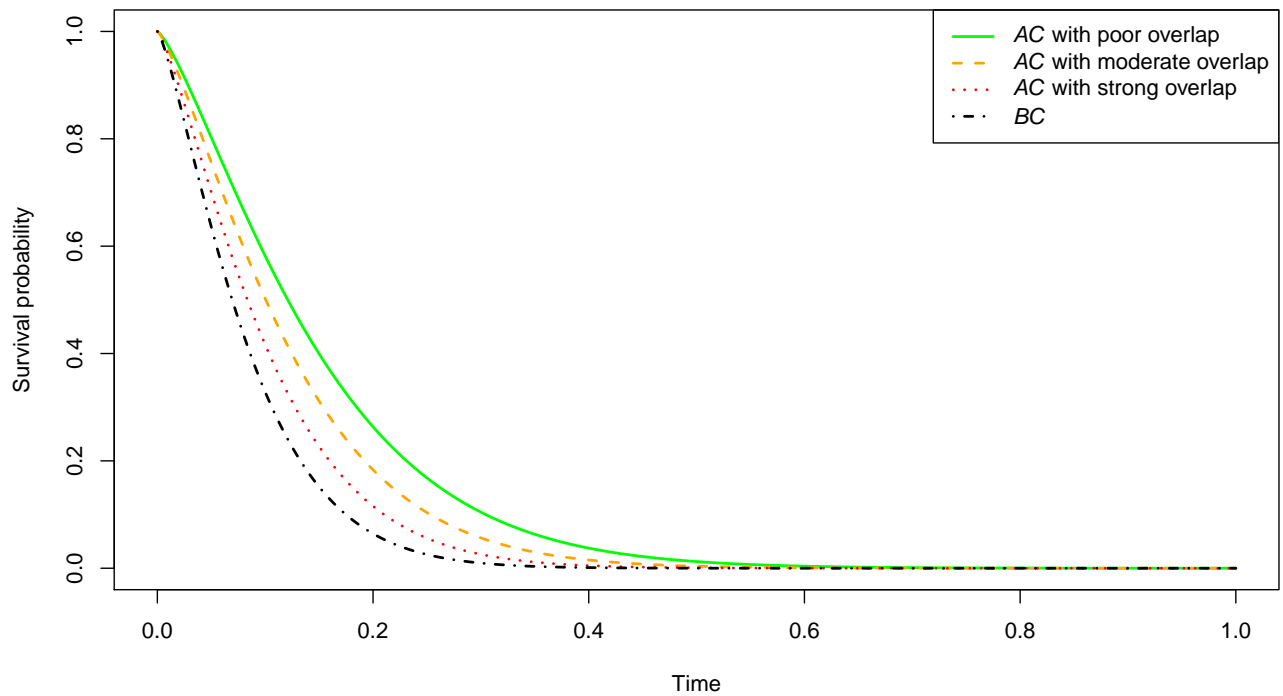

Figure 2: Weibull-distributed curves used to simulate survival times for subjects under the common comparator.



## Estimands

As per the main text.

## Methods

As per the main text.

## Performance measures

We generate and analyze 1,000 Monte Carlo replicates of trial data per simulation scenario. Let  $\hat{\Delta}_{AB,s}^*$  denote the estimator for the  $s$ -th Monte Carlo replicate and let  $\mathbb{E}(\hat{\Delta}_{AB}^*)$  denote its mean across the 1,000 simulations.

Based on a test run of the method and simulation scenario with the highest long-run variability (MAIC under Scenario 109), we assume that  $\text{SD}(\hat{\Delta}_{AB}^*) \leq 0.45$  and that, conservatively, the variance across simulations of the estimated treatment effect is always less than approximately 0.2. Given that the MCSE of the bias is equal to  $\sqrt{\text{Var}(\hat{\Delta}_{AB}^*)/N_{sim}}$ , it is at most 0.014 under 1,000 simulations. We consider the degree of precision provided by the MCSE to be acceptable in relation to the size of the effects. If the empirical coverage rate of the methods is 95%,  $N_{sim} = 1000$  implies that the MCSE of the coverage is  $\sqrt{(95 \times 5)/1000} = 0.475\%$ , with the worst-case MCSE being 2.5% under 50% coverage. We also consider this degree of precision to be acceptable. Hence, the simulation study is conducted under  $N_{sim} = 1000$ .

The criteria below are considered jointly to assess the methods' performances. Monte Carlo standard errors (MCSEs) are estimated for each performance metric in order to quantify the simulation uncertainty due to using a finite number of simulation replicates.

- To assess aim 1, we compute the **bias** in the estimated treatment effect. The bias is estimated as  $\mathbb{E}(\hat{\Delta}_{AB}^* - \Delta_{AB}^*) = \frac{1}{1000} \sum_{s=1}^{1000} \hat{\Delta}_{AB,s}^* - \Delta_{AB}^*$ . As  $\Delta_{AB}^* = 0$ , the bias is equal to the average treatment effect across the simulations. The MCSE of the bias is estimated as  $\sqrt{\frac{1}{1000 \times 999} \sum_{s=1}^{1000} (\hat{\Delta}_{AB,s}^* - \mathbb{E}(\hat{\Delta}_{AB}^*))^2}$ .
- To assess aim 2, we calculate the **variability ratio** of the treatment effect estimate. This metric is defined as the ratio of the average standard error and the observed standard deviation (empirical standard error):  $\frac{\frac{1}{1000} \sum_{s=1}^{1000} \sqrt{\hat{V}(\hat{\Delta}_{AB,s}^*)}}{\sqrt{\frac{1}{999} \sum_{s=1}^{1000} (\hat{\Delta}_{AB,s}^* - \mathbb{E}(\hat{\Delta}_{AB}^*))^2}}$ . A ratio above 1 (or below 1) suggests that, on average, standard errors overestimate (or underestimate) the variability of the treatment effect estimate. The MCSE of the variability ratio is approximated as  $\sqrt{\frac{\frac{1}{1000} \sum_{j=1}^{1000} \left( \sqrt{\hat{V}(\hat{\Delta}_{AB,j}^*)} - \mathbb{E}(\sqrt{\hat{V}(\hat{\Delta}_{AB}^*)}) \right)^2}{999 \times \widehat{ESE}^2} + \frac{\left( \frac{1}{1000} \sum_{j=1}^{1000} \sqrt{\hat{V}(\hat{\Delta}_{AB,j}^*)} \right)^2}{2 \times 999 \times \widehat{ESE}^2}}$ , where  $\widehat{ESE}$  is the estimated empirical standard error (see below).
- Aim 3 is assessed using the **coverage** of confidence intervals. This measure is estimated as the proportion of times that the true treatment effect is enclosed in the  $(100 \times (1 - \alpha))\%$  confidence interval of the estimated treatment effect, where  $\alpha = 0.05$  is the nominal significance level. The MCSE of the coverage is computed as  $\sqrt{\frac{\widehat{Cov} \times (1 - \widehat{Cov})}{1000}}$ , where  $\widehat{Cov}$  is the estimated coverage.
- We use **empirical standard error** (ESE) to assess aim 4 as it measures the precision or long-run variability of the treatment effect estimate. ESE is estimated as the standard deviation of  $\hat{\Delta}_{AB}^*$  across the 1,000 replicates:  $\sqrt{\frac{1}{999} \sum_{s=1}^{1000} (\hat{\Delta}_{AB,s}^* - \mathbb{E}(\hat{\Delta}_{AB}^*))^2}$ . The MCSE of the empirical standard error is estimated as  $\frac{\widehat{ESE}}{\sqrt{2 \times 999}}$ .
- The **mean square error** (MSE) of the estimated treatment effect. The MSE is estimated as  $\mathbb{E}[(\hat{\Delta}_{AB}^* - \Delta_{AB}^*)^2] = \frac{1}{1000} \sum_{s=1}^{1000} (\hat{\Delta}_{AB,s}^* - \Delta_{AB}^*)^2$ . The MSE provides a summary value of overall accuracy (efficiency), integrating elements of both bias (aim 1) and variability (aim 4): it can be written as the sum of the

variance and the squared bias of the estimator. The Monte Carlo standard error of the MSE is computed as

$$\sqrt{\frac{\sum_{s=1}^{1000} \left[ (\hat{\Delta}_{AB,s}^* - \Delta_{AB}^*)^2 - \widehat{MSE} \right]^2}{1000 \times 999}}, \text{ where } \widehat{MSE} \text{ is the estimated mean square error.}$$

- The **mean absolute error** (MAE) of the estimated treatment effect. The MAE is estimated as  $\frac{1}{1000} \sum_{s=1}^{1000} |\hat{\Delta}_{AB,s}^* - \Delta_{AB}^*|$ . The MAE provides another summary value of overall accuracy or efficiency. The

Monte Carlo standard error of the MAE is estimated as  $\sqrt{\frac{\sum_{s=1}^{1000} \left[ |\hat{\Delta}_{AB,s}^* - \Delta_{AB}^*| - \widehat{MAE} \right]^2}{1000 \times 999}}$ , where  $\widehat{MAE}$  is the estimated mean absolute error.

The impact of the bias on performance will depend on the uncertainty in the estimated treatment effect. To assess such impact, the **standardized bias** is estimated by computing the bias as a percentage of the empirical standard error:  $\frac{\frac{1}{1000} \sum_{s=1}^{1000} \hat{\Delta}_{AB,s}^* - \Delta_{AB}^*}{\widehat{ESE}} \times 100$ .

Apart from the performance metrics above, for each simulation scenario we track: average 95% confidence interval widths, the proportion of replicates “worse”, i.e., with point estimates that are further away from the true treatment effect, than the Bucher method (for MAIC and STC), and approximate effective sample sizes for MAIC.

## Appendix C: Scenario settings

In Table 2, parameter values for each scenario are presented.

Table 2: Parameter values for the simulation study scenarios.

| Scenario | Number of subjects in $AC$ | Prognostic effect | Interaction effect | Mean of $AC$ covariates | Covariate correlation |
|----------|----------------------------|-------------------|--------------------|-------------------------|-----------------------|
| 1        | 150                        | 0.40              | 0.40               | 0.45                    | 0.00                  |
| 2        | 300                        | 0.40              | 0.40               | 0.45                    | 0.00                  |
| 3        | 600                        | 0.40              | 0.40               | 0.45                    | 0.00                  |
| 4        | 150                        | 0.69              | 0.40               | 0.45                    | 0.00                  |
| 5        | 300                        | 0.69              | 0.40               | 0.45                    | 0.00                  |
| 6        | 600                        | 0.69              | 0.40               | 0.45                    | 0.00                  |
| 7        | 150                        | 1.11              | 0.40               | 0.45                    | 0.00                  |
| 8        | 300                        | 1.11              | 0.40               | 0.45                    | 0.00                  |
| 9        | 600                        | 1.11              | 0.40               | 0.45                    | 0.00                  |
| 10       | 150                        | 0.40              | 0.69               | 0.45                    | 0.00                  |
| 11       | 300                        | 0.40              | 0.69               | 0.45                    | 0.00                  |
| 12       | 600                        | 0.40              | 0.69               | 0.45                    | 0.00                  |
| 13       | 150                        | 0.69              | 0.69               | 0.45                    | 0.00                  |
| 14       | 300                        | 0.69              | 0.69               | 0.45                    | 0.00                  |
| 15       | 600                        | 0.69              | 0.69               | 0.45                    | 0.00                  |
| 16       | 150                        | 1.11              | 0.69               | 0.45                    | 0.00                  |
| 17       | 300                        | 1.11              | 0.69               | 0.45                    | 0.00                  |
| 18       | 600                        | 1.11              | 0.69               | 0.45                    | 0.00                  |
| 19       | 150                        | 0.40              | 1.11               | 0.45                    | 0.00                  |
| 20       | 300                        | 0.40              | 1.11               | 0.45                    | 0.00                  |
| 21       | 600                        | 0.40              | 1.11               | 0.45                    | 0.00                  |
| 22       | 150                        | 0.69              | 1.11               | 0.45                    | 0.00                  |
| 23       | 300                        | 0.69              | 1.11               | 0.45                    | 0.00                  |
| 24       | 600                        | 0.69              | 1.11               | 0.45                    | 0.00                  |
| 25       | 150                        | 1.11              | 1.11               | 0.45                    | 0.00                  |
| 26       | 300                        | 1.11              | 1.11               | 0.45                    | 0.00                  |
| 27       | 600                        | 1.11              | 1.11               | 0.45                    | 0.00                  |
| 28       | 150                        | 0.40              | 0.40               | 0.45                    | 0.35                  |
| 29       | 300                        | 0.40              | 0.40               | 0.45                    | 0.35                  |
| 30       | 600                        | 0.40              | 0.40               | 0.45                    | 0.35                  |
| 31       | 150                        | 0.69              | 0.40               | 0.45                    | 0.35                  |
| 32       | 300                        | 0.69              | 0.40               | 0.45                    | 0.35                  |
| 33       | 600                        | 0.69              | 0.40               | 0.45                    | 0.35                  |
| 34       | 150                        | 1.11              | 0.40               | 0.45                    | 0.35                  |
| 35       | 300                        | 1.11              | 0.40               | 0.45                    | 0.35                  |
| 36       | 600                        | 1.11              | 0.40               | 0.45                    | 0.35                  |
| 37       | 150                        | 0.40              | 0.69               | 0.45                    | 0.35                  |
| 38       | 300                        | 0.40              | 0.69               | 0.45                    | 0.35                  |
| 39       | 600                        | 0.40              | 0.69               | 0.45                    | 0.35                  |
| 40       | 150                        | 0.69              | 0.69               | 0.45                    | 0.35                  |
| 41       | 300                        | 0.69              | 0.69               | 0.45                    | 0.35                  |
| 42       | 600                        | 0.69              | 0.69               | 0.45                    | 0.35                  |
| 43       | 150                        | 1.11              | 0.69               | 0.45                    | 0.35                  |
| 44       | 300                        | 1.11              | 0.69               | 0.45                    | 0.35                  |
| 45       | 600                        | 1.11              | 0.69               | 0.45                    | 0.35                  |
| 46       | 150                        | 0.40              | 1.11               | 0.45                    | 0.35                  |
| 47       | 300                        | 0.40              | 1.11               | 0.45                    | 0.35                  |
| 48       | 600                        | 0.40              | 1.11               | 0.45                    | 0.35                  |
| 49       | 150                        | 0.69              | 1.11               | 0.45                    | 0.35                  |
| 50       | 300                        | 0.69              | 1.11               | 0.45                    | 0.35                  |
| 51       | 600                        | 0.69              | 1.11               | 0.45                    | 0.35                  |
| 52       | 150                        | 1.11              | 1.11               | 0.45                    | 0.35                  |
| 53       | 300                        | 1.11              | 1.11               | 0.45                    | 0.35                  |
| 54       | 600                        | 1.11              | 1.11               | 0.45                    | 0.35                  |
| 55       | 150                        | 0.40              | 0.40               | 0.30                    | 0.00                  |
| 56       | 300                        | 0.40              | 0.40               | 0.30                    | 0.00                  |
| 57       | 600                        | 0.40              | 0.40               | 0.30                    | 0.00                  |
| 58       | 150                        | 0.69              | 0.40               | 0.30                    | 0.00                  |
| 59       | 300                        | 0.69              | 0.40               | 0.30                    | 0.00                  |
| 60       | 600                        | 0.69              | 0.40               | 0.30                    | 0.00                  |
| 61       | 150                        | 1.11              | 0.40               | 0.30                    | 0.00                  |
| 62       | 300                        | 1.11              | 0.40               | 0.30                    | 0.00                  |
| 63       | 600                        | 1.11              | 0.40               | 0.30                    | 0.00                  |

Table 2: Parameter values for the simulation study scenarios. (*continued*)

| Scenario | Number of subjects in<br>$AC$ | Prognostic effect | Interaction effect | Mean of $AC$ covariates | Covariate correlation |
|----------|-------------------------------|-------------------|--------------------|-------------------------|-----------------------|
| 64       | 150                           | 0.40              | 0.69               | 0.30                    | 0.00                  |
| 65       | 300                           | 0.40              | 0.69               | 0.30                    | 0.00                  |
| 66       | 600                           | 0.40              | 0.69               | 0.30                    | 0.00                  |
| 67       | 150                           | 0.69              | 0.69               | 0.30                    | 0.00                  |
| 68       | 300                           | 0.69              | 0.69               | 0.30                    | 0.00                  |
| 69       | 600                           | 0.69              | 0.69               | 0.30                    | 0.00                  |
| 70       | 150                           | 1.11              | 0.69               | 0.30                    | 0.00                  |
| 71       | 300                           | 1.11              | 0.69               | 0.30                    | 0.00                  |
| 72       | 600                           | 1.11              | 0.69               | 0.30                    | 0.00                  |
| 73       | 150                           | 0.40              | 1.11               | 0.30                    | 0.00                  |
| 74       | 300                           | 0.40              | 1.11               | 0.30                    | 0.00                  |
| 75       | 600                           | 0.40              | 1.11               | 0.30                    | 0.00                  |
| 76       | 150                           | 0.69              | 1.11               | 0.30                    | 0.00                  |
| 77       | 300                           | 0.69              | 1.11               | 0.30                    | 0.00                  |
| 78       | 600                           | 0.69              | 1.11               | 0.30                    | 0.00                  |
| 79       | 150                           | 1.11              | 1.11               | 0.30                    | 0.00                  |
| 80       | 300                           | 1.11              | 1.11               | 0.30                    | 0.00                  |
| 81       | 600                           | 1.11              | 1.11               | 0.30                    | 0.00                  |
| 82       | 150                           | 0.40              | 0.40               | 0.30                    | 0.35                  |
| 83       | 300                           | 0.40              | 0.40               | 0.30                    | 0.35                  |
| 84       | 600                           | 0.40              | 0.40               | 0.30                    | 0.35                  |
| 85       | 150                           | 0.69              | 0.40               | 0.30                    | 0.35                  |
| 86       | 300                           | 0.69              | 0.40               | 0.30                    | 0.35                  |
| 87       | 600                           | 0.69              | 0.40               | 0.30                    | 0.35                  |
| 88       | 150                           | 1.11              | 0.40               | 0.30                    | 0.35                  |
| 89       | 300                           | 1.11              | 0.40               | 0.30                    | 0.35                  |
| 90       | 600                           | 1.11              | 0.40               | 0.30                    | 0.35                  |
| 91       | 150                           | 0.40              | 0.69               | 0.30                    | 0.35                  |
| 92       | 300                           | 0.40              | 0.69               | 0.30                    | 0.35                  |
| 93       | 600                           | 0.40              | 0.69               | 0.30                    | 0.35                  |
| 94       | 150                           | 0.69              | 0.69               | 0.30                    | 0.35                  |
| 95       | 300                           | 0.69              | 0.69               | 0.30                    | 0.35                  |
| 96       | 600                           | 0.69              | 0.69               | 0.30                    | 0.35                  |
| 97       | 150                           | 1.11              | 0.69               | 0.30                    | 0.35                  |
| 98       | 300                           | 1.11              | 0.69               | 0.30                    | 0.35                  |
| 99       | 600                           | 1.11              | 0.69               | 0.30                    | 0.35                  |
| 100      | 150                           | 0.40              | 1.11               | 0.30                    | 0.35                  |
| 101      | 300                           | 0.40              | 1.11               | 0.30                    | 0.35                  |
| 102      | 600                           | 0.40              | 1.11               | 0.30                    | 0.35                  |
| 103      | 150                           | 0.69              | 1.11               | 0.30                    | 0.35                  |
| 104      | 300                           | 0.69              | 1.11               | 0.30                    | 0.35                  |
| 105      | 600                           | 0.69              | 1.11               | 0.30                    | 0.35                  |
| 106      | 150                           | 1.11              | 1.11               | 0.30                    | 0.35                  |
| 107      | 300                           | 1.11              | 1.11               | 0.30                    | 0.35                  |
| 108      | 600                           | 1.11              | 1.11               | 0.30                    | 0.35                  |
| 109      | 150                           | 0.40              | 0.40               | 0.15                    | 0.00                  |
| 110      | 300                           | 0.40              | 0.40               | 0.15                    | 0.00                  |
| 111      | 600                           | 0.40              | 0.40               | 0.15                    | 0.00                  |
| 112      | 150                           | 0.69              | 0.40               | 0.15                    | 0.00                  |
| 113      | 300                           | 0.69              | 0.40               | 0.15                    | 0.00                  |
| 114      | 600                           | 0.69              | 0.40               | 0.15                    | 0.00                  |
| 115      | 150                           | 1.11              | 0.40               | 0.15                    | 0.00                  |
| 116      | 300                           | 1.11              | 0.40               | 0.15                    | 0.00                  |
| 117      | 600                           | 1.11              | 0.40               | 0.15                    | 0.00                  |
| 118      | 150                           | 0.40              | 0.69               | 0.15                    | 0.00                  |
| 119      | 300                           | 0.40              | 0.69               | 0.15                    | 0.00                  |
| 120      | 600                           | 0.40              | 0.69               | 0.15                    | 0.00                  |
| 121      | 150                           | 0.69              | 0.69               | 0.15                    | 0.00                  |
| 122      | 300                           | 0.69              | 0.69               | 0.15                    | 0.00                  |
| 123      | 600                           | 0.69              | 0.69               | 0.15                    | 0.00                  |
| 124      | 150                           | 1.11              | 0.69               | 0.15                    | 0.00                  |
| 125      | 300                           | 1.11              | 0.69               | 0.15                    | 0.00                  |
| 126      | 600                           | 1.11              | 0.69               | 0.15                    | 0.00                  |
| 127      | 150                           | 0.40              | 1.11               | 0.15                    | 0.00                  |
| 128      | 300                           | 0.40              | 1.11               | 0.15                    | 0.00                  |
| 129      | 600                           | 0.40              | 1.11               | 0.15                    | 0.00                  |
| 130      | 150                           | 0.69              | 1.11               | 0.15                    | 0.00                  |
| 131      | 300                           | 0.69              | 1.11               | 0.15                    | 0.00                  |

Table 2: Parameter values for the simulation study scenarios. (*continued*)

| Scenario | Number of subjects in<br>$AC$ | Prognostic effect | Interaction effect | Mean of $AC$ covariates | Covariate correlation |
|----------|-------------------------------|-------------------|--------------------|-------------------------|-----------------------|
| 132      | 600                           | 0.69              | 1.11               | 0.15                    | 0.00                  |
| 133      | 150                           | 1.11              | 1.11               | 0.15                    | 0.00                  |
| 134      | 300                           | 1.11              | 1.11               | 0.15                    | 0.00                  |
| 135      | 600                           | 1.11              | 1.11               | 0.15                    | 0.00                  |
| 136      | 150                           | 0.40              | 0.40               | 0.15                    | 0.35                  |
| 137      | 300                           | 0.40              | 0.40               | 0.15                    | 0.35                  |
| 138      | 600                           | 0.40              | 0.40               | 0.15                    | 0.35                  |
| 139      | 150                           | 0.69              | 0.40               | 0.15                    | 0.35                  |
| 140      | 300                           | 0.69              | 0.40               | 0.15                    | 0.35                  |
| 141      | 600                           | 0.69              | 0.40               | 0.15                    | 0.35                  |
| 142      | 150                           | 1.11              | 0.40               | 0.15                    | 0.35                  |
| 143      | 300                           | 1.11              | 0.40               | 0.15                    | 0.35                  |
| 144      | 600                           | 1.11              | 0.40               | 0.15                    | 0.35                  |
| 145      | 150                           | 0.40              | 0.69               | 0.15                    | 0.35                  |
| 146      | 300                           | 0.40              | 0.69               | 0.15                    | 0.35                  |
| 147      | 600                           | 0.40              | 0.69               | 0.15                    | 0.35                  |
| 148      | 150                           | 0.69              | 0.69               | 0.15                    | 0.35                  |
| 149      | 300                           | 0.69              | 0.69               | 0.15                    | 0.35                  |
| 150      | 600                           | 0.69              | 0.69               | 0.15                    | 0.35                  |
| 151      | 150                           | 1.11              | 0.69               | 0.15                    | 0.35                  |
| 152      | 300                           | 1.11              | 0.69               | 0.15                    | 0.35                  |
| 153      | 600                           | 1.11              | 0.69               | 0.15                    | 0.35                  |
| 154      | 150                           | 0.40              | 1.11               | 0.15                    | 0.35                  |
| 155      | 300                           | 0.40              | 1.11               | 0.15                    | 0.35                  |
| 156      | 600                           | 0.40              | 1.11               | 0.15                    | 0.35                  |
| 157      | 150                           | 0.69              | 1.11               | 0.15                    | 0.35                  |
| 158      | 300                           | 0.69              | 1.11               | 0.15                    | 0.35                  |
| 159      | 600                           | 0.69              | 1.11               | 0.15                    | 0.35                  |
| 160      | 150                           | 1.11              | 1.11               | 0.15                    | 0.35                  |
| 161      | 300                           | 1.11              | 1.11               | 0.15                    | 0.35                  |
| 162      | 600                           | 1.11              | 1.11               | 0.15                    | 0.35                  |

## Appendix D: Simulation study results

Table 3 displays the key performance measures associated with each of the simulated scenarios. Biases are displayed in **red** when their absolute size is greater than one half of the treatment effect estimate’s empirical standard error. Coverage rates are presented in **red** when these are statistically significantly different to 0.95; namely, if the rate is less than 0.9365 or more than 0.9635. Monte Carlo standard errors for each measure are presented in parentheses.

Table 3: Performance metrics for each method and simulation scenario. Monte Carlo standard errors for each measure are presented in parentheses. ATE: average estimated marginal treatment effect for  $A$  vs.  $B$  (is equal to the bias as the true effect is zero); LCI: average lower bound of the 95 percent confidence interval; UCI: average upper bound of the 95 percent confidence interval; MSE: mean square error; MAE: mean absolute error; Cov: coverage rate of the 95 percent confidence intervals; VR: variability ratio; ESE: empirical standard error; MAIC: matching-adjusted indirect comparison; STC: simulated treatment comparison.

| Scenario | Method | ATE                   | LCI            | UCI           | MSE           | MAE           | Cov                  | VR            | ESE           |
|----------|--------|-----------------------|----------------|---------------|---------------|---------------|----------------------|---------------|---------------|
| 1        | MAIC   | -0.010 (0.007)        | -0.429 (0.007) | 0.410 (0.007) | 0.046 (0.002) | 0.170 (0.007) | 0.950 (0.007)        | 1.001 (0.022) | 0.214 (0.005) |
| 1        | STC    | -0.065 (0.007)        | -0.513 (0.008) | 0.383 (0.007) | 0.059 (0.003) | 0.195 (0.007) | 0.938 (0.008)        | 0.974 (0.022) | 0.235 (0.005) |
| 1        | Bucher | -0.095 (0.007)        | -0.504 (0.007) | 0.315 (0.006) | 0.054 (0.002) | 0.187 (0.007) | <b>0.927 (0.008)</b> | 0.985 (0.022) | 0.212 (0.005) |
| 2        | MAIC   | 0.010 (0.005)         | -0.310 (0.005) | 0.331 (0.005) | 0.026 (0.001) | 0.129 (0.005) | 0.955 (0.007)        | 1.020 (0.023) | 0.160 (0.004) |
| 2        | STC    | -0.034 (0.005)        | -0.369 (0.005) | 0.300 (0.005) | 0.030 (0.001) | 0.140 (0.005) | 0.950 (0.007)        | 1.006 (0.023) | 0.170 (0.004) |
| 2        | Bucher | -0.075 (0.005)        | -0.390 (0.005) | 0.239 (0.005) | 0.031 (0.001) | 0.141 (0.005) | <b>0.928 (0.008)</b> | 1.007 (0.023) | 0.159 (0.004) |
| 3        | MAIC   | -0.009 (0.004)        | -0.267 (0.004) | 0.250 (0.004) | 0.018 (0.001) | 0.108 (0.004) | 0.939 (0.008)        | 0.975 (0.022) | 0.135 (0.003) |
| 3        | STC    | -0.046 (0.004)        | -0.312 (0.004) | 0.220 (0.004) | 0.022 (0.001) | 0.120 (0.004) | <b>0.924 (0.008)</b> | 0.964 (0.022) | 0.141 (0.003) |
| 3        | Bucher | <b>-0.092 (0.004)</b> | -0.347 (0.004) | 0.162 (0.004) | 0.026 (0.001) | 0.129 (0.004) | <b>0.883 (0.010)</b> | 0.977 (0.022) | 0.133 (0.003) |
| 4        | MAIC   | -0.007 (0.007)        | -0.407 (0.007) | 0.393 (0.006) | 0.043 (0.002) | 0.163 (0.007) | 0.940 (0.008)        | 0.981 (0.022) | 0.208 (0.005) |
| 4        | STC    | -0.111 (0.007)        | -0.549 (0.007) | 0.328 (0.007) | 0.065 (0.003) | 0.200 (0.007) | <b>0.918 (0.009)</b> | 0.974 (0.022) | 0.230 (0.005) |
| 4        | Bucher | -0.081 (0.007)        | -0.478 (0.007) | 0.316 (0.006) | 0.049 (0.002) | 0.176 (0.007) | <b>0.935 (0.008)</b> | 0.983 (0.022) | 0.206 (0.005) |
| 5        | MAIC   | 0.006 (0.005)         | -0.301 (0.005) | 0.312 (0.005) | 0.024 (0.001) | 0.122 (0.005) | 0.941 (0.007)        | 1.003 (0.022) | 0.156 (0.003) |
| 5        | STC    | <b>-0.093 (0.005)</b> | -0.419 (0.005) | 0.234 (0.005) | 0.037 (0.002) | 0.152 (0.005) | <b>0.913 (0.009)</b> | 0.986 (0.022) | 0.169 (0.004) |
| 5        | Bucher | -0.072 (0.005)        | -0.378 (0.005) | 0.233 (0.005) | 0.030 (0.001) | 0.136 (0.005) | <b>0.920 (0.009)</b> | 1.000 (0.022) | 0.156 (0.003) |
| 6        | MAIC   | 0.002 (0.004)         | -0.247 (0.004) | 0.251 (0.004) | 0.016 (0.001) | 0.100 (0.004) | 0.943 (0.007)        | 1.001 (0.022) | 0.127 (0.003) |
| 6        | STC    | <b>-0.087 (0.004)</b> | -0.346 (0.004) | 0.173 (0.004) | 0.025 (0.001) | 0.127 (0.004) | <b>0.901 (0.009)</b> | 1.001 (0.022) | 0.132 (0.003) |
| 6        | Bucher | <b>-0.076 (0.004)</b> | -0.324 (0.004) | 0.172 (0.004) | 0.022 (0.001) | 0.119 (0.004) | <b>0.910 (0.009)</b> | 1.000 (0.022) | 0.127 (0.003) |
| 7        | MAIC   | -0.003 (0.006)        | -0.386 (0.006) | 0.379 (0.006) | 0.039 (0.002) | 0.157 (0.006) | 0.947 (0.007)        | 0.991 (0.022) | 0.197 (0.004) |
| 7        | STC    | <b>-0.184 (0.007)</b> | -0.614 (0.007) | 0.246 (0.007) | 0.082 (0.004) | 0.233 (0.007) | <b>0.873 (0.011)</b> | 0.995 (0.022) | 0.221 (0.005) |
| 7        | Bucher | -0.073 (0.006)        | -0.459 (0.006) | 0.313 (0.006) | 0.044 (0.002) | 0.165 (0.006) | <b>0.936 (0.008)</b> | 1.000 (0.022) | 0.197 (0.004) |
| 8        | MAIC   | 0.000 (0.005)         | -0.295 (0.005) | 0.294 (0.005) | 0.023 (0.001) | 0.122 (0.005) | 0.954 (0.007)        | 0.995 (0.022) | 0.151 (0.003) |
| 8        | STC    | <b>-0.174 (0.005)</b> | -0.494 (0.005) | 0.146 (0.005) | 0.058 (0.002) | 0.197 (0.005) | <b>0.817 (0.012)</b> | 0.982 (0.022) | 0.166 (0.004) |
| 8        | Bucher | -0.068 (0.005)        | -0.364 (0.005) | 0.229 (0.005) | 0.028 (0.001) | 0.133 (0.005) | <b>0.925 (0.008)</b> | 0.987 (0.022) | 0.153 (0.003) |
| 9        | MAIC   | 0.003 (0.004)         | -0.237 (0.004) | 0.242 (0.004) | 0.016 (0.001) | 0.102 (0.004) | 0.951 (0.007)        | 0.965 (0.022) | 0.127 (0.003) |
| 9        | STC    | <b>-0.166 (0.004)</b> | -0.420 (0.004) | 0.088 (0.004) | 0.046 (0.002) | 0.179 (0.004) | <b>0.740 (0.014)</b> | 0.966 (0.022) | 0.134 (0.003) |
| 9        | Bucher | -0.063 (0.004)        | -0.303 (0.004) | 0.178 (0.004) | 0.021 (0.001) | 0.116 (0.004) | <b>0.905 (0.009)</b> | 0.937 (0.021) | 0.131 (0.003) |
| 10       | MAIC   | 0.003 (0.006)         | -0.399 (0.006) | 0.406 (0.006) | 0.040 (0.002) | 0.160 (0.006) | 0.954 (0.007)        | 1.023 (0.023) | 0.201 (0.004) |
| 10       | STC    | -0.007 (0.007)        | -0.443 (0.007) | 0.429 (0.007) | 0.050 (0.002) | 0.179 (0.007) | 0.948 (0.007)        | 0.993 (0.022) | 0.224 (0.005) |
| 10       | Bucher | <b>-0.138 (0.006)</b> | -0.538 (0.006) | 0.261 (0.006) | 0.058 (0.003) | 0.192 (0.006) | <b>0.905 (0.009)</b> | 1.037 (0.023) | 0.197 (0.004) |
| 11       | MAIC   | 0.003 (0.005)         | -0.305 (0.005) | 0.312 (0.005) | 0.024 (0.001) | 0.123 (0.005) | 0.953 (0.007)        | 1.021 (0.023) | 0.154 (0.003) |
| 11       | STC    | 0.003 (0.005)         | -0.323 (0.005) | 0.329 (0.005) | 0.028 (0.001) | 0.134 (0.005) | 0.950 (0.007)        | 0.995 (0.022) | 0.167 (0.004) |
| 11       | Bucher | <b>-0.139 (0.005)</b> | -0.447 (0.005) | 0.168 (0.005) | 0.044 (0.002) | 0.172 (0.005) | <b>0.860 (0.011)</b> | 1.001 (0.022) | 0.157 (0.004) |
| 12       | MAIC   | 0.000 (0.004)         | -0.250 (0.004) | 0.250 (0.004) | 0.016 (0.001) | 0.101 (0.004) | <b>0.964 (0.006)</b> | 1.018 (0.023) | 0.125 (0.003) |
| 12       | STC    | 0.003 (0.004)         | -0.257 (0.004) | 0.262 (0.004) | 0.017 (0.001) | 0.106 (0.004) | <b>0.964 (0.006)</b> | 1.010 (0.023) | 0.131 (0.003) |
| 12       | Bucher | <b>-0.140 (0.004)</b> | -0.389 (0.004) | 0.110 (0.004) | 0.035 (0.001) | 0.156 (0.004) | <b>0.804 (0.013)</b> | 1.013 (0.023) | 0.126 (0.003) |
| 13       | MAIC   | -0.001 (0.006)        | -0.389 (0.006) | 0.387 (0.006) | 0.038 (0.002) | 0.155 (0.006) | 0.948 (0.007)        | 1.011 (0.023) | 0.196 (0.004) |
| 13       | STC    | -0.040 (0.007)        | -0.468 (0.007) | 0.387 (0.007) | 0.050 (0.002) | 0.178 (0.007) | 0.945 (0.007)        | 0.990 (0.022) | 0.220 (0.005) |
| 13       | Bucher | <b>-0.131 (0.006)</b> | -0.522 (0.007) | 0.261 (0.006) | 0.057 (0.003) | 0.190 (0.006) | <b>0.900 (0.009)</b> | 0.996 (0.022) | 0.200 (0.004) |
| 14       | MAIC   | 0.002 (0.005)         | -0.296 (0.005) | 0.300 (0.005) | 0.022 (0.001) | 0.117 (0.005) | 0.955 (0.007)        | 1.032 (0.023) | 0.147 (0.003) |
| 14       | STC    | -0.024 (0.005)        | -0.344 (0.005) | 0.295 (0.005) | 0.027 (0.001) | 0.131 (0.005) | 0.951 (0.007)        | 1.001 (0.022) | 0.163 (0.004) |
| 14       | Bucher | <b>-0.127 (0.005)</b> | -0.427 (0.005) | 0.174 (0.005) | 0.039 (0.002) | 0.162 (0.005) | <b>0.878 (0.010)</b> | 1.001 (0.022) | 0.153 (0.003) |
| 15       | MAIC   | 0.005 (0.004)         | -0.237 (0.004) | 0.248 (0.004) | 0.015 (0.001) | 0.097 (0.004) | 0.949 (0.007)        | 1.013 (0.023) | 0.122 (0.003) |
| 15       | STC    | -0.019 (0.004)        | -0.274 (0.004) | 0.235 (0.004) | 0.017 (0.001) | 0.106 (0.004) | 0.954 (0.007)        | 1.002 (0.022) | 0.130 (0.003) |
| 15       | Bucher | <b>-0.120 (0.004)</b> | -0.364 (0.004) | 0.124 (0.004) | 0.030 (0.001) | 0.141 (0.004) | <b>0.839 (0.012)</b> | 1.006 (0.023) | 0.124 (0.003) |
| 16       | MAIC   | -0.010 (0.006)        | -0.385 (0.006) | 0.366 (0.006) | 0.038 (0.002) | 0.155 (0.006) | 0.944 (0.007)        | 0.980 (0.022) | 0.195 (0.004) |
| 16       | STC    | -0.082 (0.007)        | -0.503 (0.007) | 0.339 (0.007) | 0.059 (0.003) | 0.190 (0.007) | <b>0.915 (0.009)</b> | 0.942 (0.021) | 0.228 (0.005) |
| 16       | Bucher | <b>-0.119 (0.006)</b> | -0.501 (0.006) | 0.264 (0.006) | 0.054 (0.002) | 0.185 (0.006) | <b>0.904 (0.009)</b> | 0.972 (0.022) | 0.201 (0.004) |
| 17       | MAIC   | -0.001 (0.005)        | -0.289 (0.005) | 0.288 (0.005) | 0.023 (0.001) | 0.123 (0.005) | 0.942 (0.007)        | 0.964 (0.022) | 0.153 (0.003) |
| 17       | STC    | -0.070 (0.005)        | -0.385 (0.005) | 0.244 (0.005) | 0.034 (0.002) | 0.146 (0.005) | <b>0.908 (0.009)</b> | 0.942 (0.021) | 0.170 (0.004) |
| 17       | Bucher | <b>-0.109 (0.005)</b> | -0.403 (0.005) | 0.184 (0.005) | 0.036 (0.001) | 0.154 (0.005) | <b>0.870 (0.011)</b> | 0.963 (0.022) | 0.156 (0.003) |

Table 3: Performance metrics for each method and simulation scenario. Monte Carlo standard errors for each measure are presented in parentheses. ATE: average estimated marginal treatment effect for  $A$  vs.  $B$  (is equal to the bias as the true effect is zero); LCI: average lower bound of the 95 percent confidence interval; UCI: average upper bound of the 95 percent confidence interval; MSE: mean square error; MAE: mean absolute error; Cov: coverage rate of the 95 percent confidence intervals; VR: variability ratio; ESE: empirical standard error; MAIC: matching-adjusted indirect comparison; STC: simulated treatment comparison. *(continued)*

| Scenario | Method | ATE            | LCI            | UCI           | MSE           | MAE           | Cov           | VR            | ESE           |
|----------|--------|----------------|----------------|---------------|---------------|---------------|---------------|---------------|---------------|
| 18       | MAIC   | 0.005 (0.004)  | -0.230 (0.004) | 0.241 (0.004) | 0.014 (0.001) | 0.093 (0.004) | 0.955 (0.007) | 1.033 (0.023) | 0.116 (0.003) |
| 18       | STC    | -0.063 (0.004) | -0.313 (0.004) | 0.187 (0.004) | 0.020 (0.001) | 0.113 (0.004) | 0.927 (0.008) | 1.021 (0.023) | 0.125 (0.003) |
| 18       | Bucher | -0.104 (0.004) | -0.342 (0.004) | 0.135 (0.004) | 0.025 (0.001) | 0.128 (0.004) | 0.881 (0.010) | 1.034 (0.023) | 0.118 (0.003) |
| 19       | MAIC   | 0.000 (0.006)  | -0.386 (0.006) | 0.387 (0.006) | 0.039 (0.002) | 0.157 (0.006) | 0.948 (0.007) | 0.995 (0.022) | 0.198 (0.004) |
| 19       | STC    | 0.095 (0.007)  | -0.332 (0.007) | 0.522 (0.007) | 0.062 (0.003) | 0.198 (0.007) | 0.911 (0.009) | 0.947 (0.021) | 0.230 (0.005) |
| 19       | Bucher | -0.204 (0.006) | -0.596 (0.007) | 0.187 (0.006) | 0.083 (0.003) | 0.239 (0.006) | 0.830 (0.012) | 0.983 (0.022) | 0.203 (0.005) |
| 20       | MAIC   | 0.012 (0.005)  | -0.285 (0.005) | 0.309 (0.005) | 0.021 (0.001) | 0.116 (0.005) | 0.960 (0.006) | 1.048 (0.023) | 0.145 (0.003) |
| 20       | STC    | 0.107 (0.005)  | -0.212 (0.005) | 0.427 (0.005) | 0.036 (0.002) | 0.154 (0.005) | 0.907 (0.009) | 1.034 (0.023) | 0.158 (0.004) |
| 20       | Bucher | -0.194 (0.005) | -0.495 (0.005) | 0.107 (0.005) | 0.061 (0.002) | 0.207 (0.005) | 0.777 (0.013) | 1.012 (0.023) | 0.152 (0.003) |
| 21       | MAIC   | 0.002 (0.004)  | -0.240 (0.004) | 0.243 (0.004) | 0.014 (0.001) | 0.095 (0.004) | 0.950 (0.007) | 1.029 (0.023) | 0.120 (0.003) |
| 21       | STC    | 0.102 (0.004)  | -0.152 (0.004) | 0.356 (0.004) | 0.027 (0.001) | 0.135 (0.004) | 0.897 (0.010) | 1.007 (0.023) | 0.129 (0.003) |
| 21       | Bucher | -0.203 (0.004) | -0.448 (0.004) | 0.041 (0.004) | 0.056 (0.002) | 0.208 (0.004) | 0.646 (0.015) | 1.015 (0.023) | 0.123 (0.003) |
| 22       | MAIC   | -0.009 (0.006) | -0.384 (0.006) | 0.366 (0.006) | 0.036 (0.002) | 0.152 (0.006) | 0.947 (0.007) | 1.006 (0.023) | 0.190 (0.004) |
| 22       | STC    | 0.093 (0.007)  | -0.327 (0.007) | 0.513 (0.007) | 0.058 (0.003) | 0.191 (0.007) | 0.913 (0.009) | 0.965 (0.022) | 0.222 (0.005) |
| 22       | Bucher | -0.186 (0.006) | -0.571 (0.006) | 0.199 (0.006) | 0.071 (0.003) | 0.220 (0.006) | 0.849 (0.011) | 1.026 (0.023) | 0.191 (0.004) |
| 23       | MAIC   | 0.007 (0.004)  | -0.282 (0.004) | 0.297 (0.004) | 0.020 (0.001) | 0.111 (0.004) | 0.953 (0.007) | 1.057 (0.024) | 0.140 (0.003) |
| 23       | STC    | 0.117 (0.005)  | -0.197 (0.005) | 0.431 (0.005) | 0.039 (0.002) | 0.161 (0.005) | 0.897 (0.010) | 1.010 (0.023) | 0.159 (0.004) |
| 23       | Bucher | -0.179 (0.005) | -0.475 (0.005) | 0.117 (0.005) | 0.053 (0.002) | 0.194 (0.005) | 0.792 (0.013) | 1.035 (0.023) | 0.146 (0.003) |
| 24       | MAIC   | 0.005 (0.004)  | -0.231 (0.004) | 0.241 (0.004) | 0.014 (0.001) | 0.093 (0.004) | 0.958 (0.006) | 1.035 (0.023) | 0.116 (0.003) |
| 24       | STC    | 0.116 (0.004)  | -0.135 (0.004) | 0.366 (0.004) | 0.029 (0.001) | 0.139 (0.004) | 0.851 (0.011) | 1.032 (0.023) | 0.124 (0.003) |
| 24       | Bucher | -0.182 (0.004) | -0.422 (0.004) | 0.059 (0.004) | 0.047 (0.002) | 0.188 (0.004) | 0.695 (0.015) | 1.023 (0.023) | 0.120 (0.003) |
| 25       | MAIC   | 0.004 (0.006)  | -0.362 (0.006) | 0.371 (0.006) | 0.033 (0.001) | 0.145 (0.006) | 0.956 (0.006) | 1.022 (0.023) | 0.183 (0.004) |
| 25       | STC    | 0.103 (0.007)  | -0.311 (0.007) | 0.518 (0.007) | 0.057 (0.003) | 0.191 (0.007) | 0.911 (0.009) | 0.982 (0.022) | 0.216 (0.005) |
| 25       | Bucher | -0.157 (0.006) | -0.536 (0.006) | 0.221 (0.006) | 0.062 (0.002) | 0.203 (0.006) | 0.880 (0.010) | 1.004 (0.022) | 0.192 (0.004) |
| 26       | MAIC   | 0.005 (0.005)  | -0.278 (0.005) | 0.289 (0.004) | 0.020 (0.001) | 0.113 (0.005) | 0.952 (0.007) | 1.013 (0.023) | 0.143 (0.003) |
| 26       | STC    | 0.114 (0.005)  | -0.196 (0.005) | 0.425 (0.005) | 0.039 (0.002) | 0.162 (0.005) | 0.881 (0.010) | 0.975 (0.022) | 0.163 (0.004) |
| 26       | Bucher | -0.155 (0.005) | -0.446 (0.005) | 0.137 (0.005) | 0.045 (0.002) | 0.176 (0.005) | 0.835 (0.012) | 1.034 (0.023) | 0.144 (0.003) |
| 27       | MAIC   | -0.001 (0.004) | -0.233 (0.004) | 0.230 (0.004) | 0.014 (0.001) | 0.094 (0.004) | 0.947 (0.007) | 0.991 (0.022) | 0.119 (0.003) |
| 27       | STC    | 0.104 (0.004)  | -0.143 (0.004) | 0.351 (0.004) | 0.028 (0.001) | 0.134 (0.004) | 0.867 (0.011) | 0.977 (0.022) | 0.129 (0.003) |
| 27       | Bucher | -0.161 (0.004) | -0.398 (0.004) | 0.076 (0.004) | 0.040 (0.001) | 0.171 (0.004) | 0.734 (0.014) | 1.005 (0.022) | 0.120 (0.003) |
| 28       | MAIC   | -0.006 (0.007) | -0.409 (0.007) | 0.397 (0.006) | 0.044 (0.002) | 0.167 (0.007) | 0.937 (0.008) | 0.978 (0.022) | 0.210 (0.005) |
| 28       | STC    | -0.089 (0.007) | -0.527 (0.008) | 0.349 (0.007) | 0.062 (0.003) | 0.200 (0.007) | 0.925 (0.008) | 0.959 (0.021) | 0.233 (0.005) |
| 28       | Bucher | -0.085 (0.007) | -0.494 (0.007) | 0.323 (0.007) | 0.052 (0.002) | 0.181 (0.007) | 0.935 (0.008) | 0.981 (0.022) | 0.212 (0.005) |
| 29       | MAIC   | -0.002 (0.005) | -0.312 (0.005) | 0.309 (0.005) | 0.024 (0.001) | 0.124 (0.005) | 0.955 (0.007) | 1.023 (0.023) | 0.155 (0.003) |
| 29       | STC    | -0.071 (0.005) | -0.400 (0.005) | 0.257 (0.005) | 0.032 (0.001) | 0.144 (0.005) | 0.936 (0.008) | 1.019 (0.023) | 0.164 (0.004) |
| 29       | Bucher | -0.081 (0.005) | -0.394 (0.005) | 0.233 (0.005) | 0.031 (0.001) | 0.141 (0.005) | 0.927 (0.008) | 1.027 (0.023) | 0.156 (0.003) |
| 30       | MAIC   | 0.000 (0.004)  | -0.253 (0.004) | 0.252 (0.004) | 0.016 (0.001) | 0.100 (0.004) | 0.955 (0.007) | 1.012 (0.023) | 0.127 (0.003) |
| 30       | STC    | -0.061 (0.004) | -0.324 (0.004) | 0.201 (0.004) | 0.022 (0.001) | 0.116 (0.004) | 0.918 (0.009) | 0.991 (0.022) | 0.135 (0.003) |
| 30       | Bucher | -0.079 (0.004) | -0.333 (0.004) | 0.176 (0.004) | 0.023 (0.001) | 0.121 (0.004) | 0.912 (0.009) | 1.009 (0.023) | 0.129 (0.003) |
| 31       | MAIC   | -0.012 (0.006) | -0.397 (0.006) | 0.373 (0.006) | 0.040 (0.002) | 0.159 (0.006) | 0.949 (0.007) | 0.984 (0.022) | 0.199 (0.004) |
| 31       | STC    | -0.170 (0.007) | -0.599 (0.007) | 0.258 (0.007) | 0.077 (0.003) | 0.224 (0.007) | 0.885 (0.010) | 0.998 (0.022) | 0.219 (0.005) |
| 31       | Bucher | -0.082 (0.006) | -0.479 (0.007) | 0.314 (0.006) | 0.047 (0.002) | 0.172 (0.006) | 0.932 (0.008) | 1.004 (0.022) | 0.202 (0.005) |
| 32       | MAIC   | 0.000 (0.005)  | -0.297 (0.005) | 0.296 (0.005) | 0.023 (0.001) | 0.121 (0.005) | 0.946 (0.007) | 0.994 (0.022) | 0.152 (0.003) |
| 32       | STC    | -0.149 (0.005) | -0.469 (0.005) | 0.171 (0.005) | 0.049 (0.002) | 0.184 (0.005) | 0.859 (0.011) | 0.993 (0.022) | 0.165 (0.004) |
| 32       | Bucher | -0.069 (0.005) | -0.373 (0.005) | 0.236 (0.005) | 0.028 (0.001) | 0.133 (0.005) | 0.928 (0.008) | 1.008 (0.023) | 0.154 (0.003) |
| 33       | MAIC   | 0.002 (0.004)  | -0.241 (0.004) | 0.244 (0.004) | 0.015 (0.001) | 0.100 (0.004) | 0.955 (0.007) | 1.000 (0.022) | 0.124 (0.003) |
| 33       | STC    | -0.139 (0.004) | -0.395 (0.004) | 0.117 (0.004) | 0.037 (0.001) | 0.160 (0.004) | 0.814 (0.012) | 0.979 (0.022) | 0.134 (0.003) |
| 33       | Bucher | -0.068 (0.004) | -0.315 (0.004) | 0.179 (0.004) | 0.021 (0.001) | 0.116 (0.004) | 0.917 (0.009) | 0.999 (0.022) | 0.126 (0.003) |
| 34       | MAIC   | -0.005 (0.006) | -0.374 (0.006) | 0.364 (0.006) | 0.037 (0.002) | 0.153 (0.006) | 0.942 (0.007) | 0.978 (0.022) | 0.193 (0.004) |
| 34       | STC    | -0.259 (0.007) | -0.680 (0.007) | 0.163 (0.007) | 0.118 (0.005) | 0.283 (0.007) | 0.769 (0.013) | 0.946 (0.021) | 0.227 (0.005) |
| 34       | Bucher | -0.059 (0.006) | -0.445 (0.006) | 0.327 (0.006) | 0.043 (0.002) | 0.163 (0.006) | 0.936 (0.008) | 0.987 (0.022) | 0.199 (0.004) |
| 35       | MAIC   | 0.009 (0.005)  | -0.276 (0.005) | 0.295 (0.005) | 0.021 (0.001) | 0.118 (0.005) | 0.957 (0.006) | 1.002 (0.022) | 0.146 (0.003) |
| 35       | STC    | -0.241 (0.005) | -0.557 (0.005) | 0.074 (0.005) | 0.084 (0.003) | 0.248 (0.005) | 0.677 (0.015) | 1.004 (0.022) | 0.160 (0.004) |
| 35       | Bucher | -0.045 (0.005) | -0.342 (0.005) | 0.252 (0.005) | 0.024 (0.001) | 0.126 (0.005) | 0.940 (0.008) | 1.016 (0.023) | 0.149 (0.003) |
| 36       | MAIC   | -0.001 (0.004) | -0.235 (0.004) | 0.234 (0.004) | 0.015 (0.001) | 0.097 (0.004) | 0.936 (0.008) | 0.982 (0.022) | 0.122 (0.003) |
| 36       | STC    | -0.243 (0.004) | -0.494 (0.004) | 0.008 (0.004) | 0.076 (0.002) | 0.246 (0.004) | 0.507 (0.016) | 0.994 (0.022) | 0.129 (0.003) |
| 36       | Bucher | -0.055 (0.004) | -0.296 (0.004) | 0.186 (0.004) | 0.019 (0.001) | 0.110 (0.004) | 0.921 (0.009) | 0.980 (0.022) | 0.125 (0.003) |
| 37       | MAIC   | -0.005 (0.006) | -0.396 (0.007) | 0.386 (0.006) | 0.041 (0.002) | 0.157 (0.006) | 0.941 (0.007) | 0.987 (0.022) | 0.202 (0.005) |
| 37       | STC    | -0.018 (0.008) | -0.446 (0.008) | 0.410 (0.007) | 0.057 (0.003) | 0.186 (0.008) | 0.919 (0.009) | 0.919 (0.021) | 0.238 (0.005) |
| 37       | Bucher | -0.136 (0.006) | -0.537 (0.007) | 0.266 (0.006) | 0.060 (0.003) | 0.194 (0.006) | 0.900 (0.009) | 1.001 (0.022) | 0.204 (0.005) |

Table 3: Performance metrics for each method and simulation scenario. Monte Carlo standard errors for each measure are presented in parentheses. ATE: average estimated marginal treatment effect for  $A$  vs.  $B$  (is equal to the bias as the true effect is zero); LCI: average lower bound of the 95 percent confidence interval; UCI: average upper bound of the 95 percent confidence interval; MSE: mean square error; MAE: mean absolute error; Cov: coverage rate of the 95 percent confidence intervals; VR: variability ratio; ESE: empirical standard error; MAIC: matching-adjusted indirect comparison; STC: simulated treatment comparison. (*continued*)

| Scenario | Method | ATE                   | LCI            | UCI           | MSE           | MAE           | Cov                  | VR            | ESE           |
|----------|--------|-----------------------|----------------|---------------|---------------|---------------|----------------------|---------------|---------------|
| 38       | MAIC   | 0.003 (0.005)         | -0.298 (0.005) | 0.304 (0.005) | 0.022 (0.001) | 0.120 (0.005) | 0.961 (0.006)        | 1.024 (0.023) | 0.150 (0.003) |
| 38       | STC    | -0.004 (0.005)        | -0.324 (0.005) | 0.317 (0.005) | 0.026 (0.001) | 0.130 (0.005) | 0.950 (0.007)        | 1.005 (0.022) | 0.163 (0.004) |
| 38       | Bucher | <b>-0.125 (0.005)</b> | -0.433 (0.005) | 0.183 (0.005) | 0.039 (0.002) | 0.161 (0.005) | <b>0.875 (0.010)</b> | 1.029 (0.023) | 0.153 (0.003) |
| 39       | MAIC   | -0.001 (0.004)        | -0.247 (0.004) | 0.244 (0.004) | 0.014 (0.001) | 0.095 (0.004) | 0.955 (0.007)        | 1.048 (0.023) | 0.120 (0.003) |
| 39       | STC    | -0.002 (0.004)        | -0.258 (0.004) | 0.255 (0.004) | 0.016 (0.001) | 0.103 (0.004) | <b>0.966 (0.006)</b> | 1.024 (0.023) | 0.128 (0.003) |
| 39       | Bucher | <b>-0.130 (0.004)</b> | -0.380 (0.004) | 0.120 (0.004) | 0.032 (0.001) | 0.148 (0.004) | <b>0.841 (0.012)</b> | 1.043 (0.023) | 0.122 (0.003) |
| 40       | MAIC   | -0.015 (0.006)        | -0.393 (0.006) | 0.362 (0.006) | 0.038 (0.002) | 0.157 (0.006) | 0.950 (0.007)        | 0.990 (0.022) | 0.195 (0.004) |
| 40       | STC    | -0.059 (0.007)        | -0.479 (0.007) | 0.360 (0.007) | 0.055 (0.002) | 0.187 (0.007) | <b>0.928 (0.008)</b> | 0.946 (0.021) | 0.226 (0.005) |
| 40       | Bucher | <b>-0.126 (0.006)</b> | -0.519 (0.007) | 0.266 (0.006) | 0.057 (0.002) | 0.189 (0.006) | <b>0.900 (0.009)</b> | 0.992 (0.022) | 0.202 (0.005) |
| 41       | MAIC   | 0.000 (0.004)         | -0.291 (0.005) | 0.291 (0.004) | 0.020 (0.001) | 0.114 (0.004) | <b>0.969 (0.005)</b> | 1.047 (0.023) | 0.142 (0.003) |
| 41       | STC    | -0.045 (0.005)        | -0.360 (0.005) | 0.270 (0.005) | 0.027 (0.001) | 0.129 (0.005) | 0.947 (0.007)        | 1.021 (0.023) | 0.157 (0.004) |
| 41       | Bucher | <b>-0.109 (0.005)</b> | -0.410 (0.005) | 0.192 (0.005) | 0.033 (0.001) | 0.147 (0.005) | <b>0.900 (0.009)</b> | 1.049 (0.023) | 0.147 (0.003) |
| 42       | MAIC   | 0.006 (0.004)         | -0.233 (0.004) | 0.244 (0.004) | 0.014 (0.001) | 0.096 (0.004) | 0.946 (0.007)        | 1.012 (0.023) | 0.120 (0.003) |
| 42       | STC    | -0.037 (0.004)        | -0.288 (0.004) | 0.215 (0.004) | 0.018 (0.001) | 0.109 (0.004) | 0.939 (0.008)        | 0.992 (0.022) | 0.129 (0.003) |
| 42       | Bucher | <b>-0.103 (0.004)</b> | -0.347 (0.004) | 0.142 (0.004) | 0.026 (0.001) | 0.131 (0.004) | <b>0.875 (0.010)</b> | 1.001 (0.022) | 0.125 (0.003) |
| 43       | MAIC   | 0.004 (0.006)         | -0.362 (0.006) | 0.370 (0.006) | 0.037 (0.002) | 0.153 (0.006) | 0.947 (0.007)        | 0.969 (0.022) | 0.193 (0.004) |
| 43       | STC    | <b>-0.114 (0.007)</b> | -0.529 (0.007) | 0.301 (0.007) | 0.060 (0.003) | 0.192 (0.007) | <b>0.904 (0.009)</b> | 0.975 (0.022) | 0.217 (0.005) |
| 43       | Bucher | -0.085 (0.006)        | -0.469 (0.006) | 0.299 (0.006) | 0.047 (0.002) | 0.173 (0.006) | <b>0.927 (0.008)</b> | 0.979 (0.022) | 0.200 (0.004) |
| 44       | MAIC   | 0.008 (0.004)         | -0.275 (0.004) | 0.292 (0.004) | 0.019 (0.001) | 0.111 (0.004) | 0.954 (0.007)        | 1.042 (0.023) | 0.139 (0.003) |
| 44       | STC    | <b>-0.102 (0.005)</b> | -0.412 (0.005) | 0.209 (0.005) | 0.037 (0.002) | 0.153 (0.005) | <b>0.905 (0.009)</b> | 0.976 (0.022) | 0.162 (0.004) |
| 44       | Bucher | <b>-0.081 (0.005)</b> | -0.376 (0.005) | 0.214 (0.005) | 0.028 (0.001) | 0.133 (0.005) | <b>0.927 (0.008)</b> | 1.027 (0.023) | 0.147 (0.003) |
| 45       | MAIC   | 0.000 (0.004)         | -0.232 (0.004) | 0.233 (0.004) | 0.014 (0.001) | 0.095 (0.004) | 0.951 (0.007)        | 1.007 (0.023) | 0.118 (0.003) |
| 45       | STC    | <b>-0.101 (0.004)</b> | -0.349 (0.004) | 0.146 (0.004) | 0.027 (0.001) | 0.132 (0.004) | <b>0.861 (0.011)</b> | 0.987 (0.022) | 0.128 (0.003) |
| 45       | Bucher | <b>-0.087 (0.004)</b> | -0.327 (0.004) | 0.152 (0.004) | 0.022 (0.001) | 0.122 (0.004) | <b>0.886 (0.010)</b> | 1.005 (0.022) | 0.122 (0.003) |
| 46       | MAIC   | 0.006 (0.006)         | -0.374 (0.006) | 0.386 (0.006) | 0.040 (0.002) | 0.160 (0.006) | 0.951 (0.007)        | 0.974 (0.022) | 0.199 (0.004) |
| 46       | STC    | <b>0.132 (0.007)</b>  | -0.289 (0.007) | 0.553 (0.007) | 0.069 (0.003) | 0.213 (0.007) | <b>0.893 (0.010)</b> | 0.942 (0.021) | 0.228 (0.005) |
| 46       | Bucher | <b>-0.182 (0.007)</b> | -0.576 (0.007) | 0.213 (0.006) | 0.076 (0.003) | 0.223 (0.007) | <b>0.844 (0.011)</b> | 0.971 (0.022) | 0.207 (0.005) |
| 47       | MAIC   | -0.006 (0.005)        | -0.299 (0.005) | 0.287 (0.005) | 0.021 (0.001) | 0.118 (0.005) | 0.960 (0.006)        | 1.021 (0.023) | 0.147 (0.003) |
| 47       | STC    | <b>0.120 (0.005)</b>  | -0.196 (0.005) | 0.436 (0.005) | 0.041 (0.002) | 0.163 (0.005) | <b>0.881 (0.010)</b> | 0.994 (0.022) | 0.162 (0.004) |
| 47       | Bucher | <b>-0.193 (0.005)</b> | -0.497 (0.005) | 0.110 (0.005) | 0.061 (0.002) | 0.210 (0.005) | <b>0.761 (0.013)</b> | 1.012 (0.023) | 0.153 (0.003) |
| 48       | MAIC   | -0.001 (0.004)        | -0.240 (0.004) | 0.239 (0.004) | 0.015 (0.001) | 0.099 (0.004) | 0.956 (0.006)        | 0.993 (0.022) | 0.123 (0.003) |
| 48       | STC    | <b>0.126 (0.004)</b>  | -0.126 (0.004) | 0.379 (0.004) | 0.033 (0.001) | 0.150 (0.004) | <b>0.827 (0.012)</b> | 0.978 (0.022) | 0.132 (0.003) |
| 48       | Bucher | <b>-0.186 (0.004)</b> | -0.433 (0.004) | 0.060 (0.004) | 0.051 (0.002) | 0.195 (0.004) | <b>0.665 (0.015)</b> | 0.969 (0.022) | 0.130 (0.003) |
| 49       | MAIC   | 0.005 (0.006)         | -0.364 (0.006) | 0.375 (0.006) | 0.034 (0.002) | 0.146 (0.006) | 0.955 (0.007)        | 1.027 (0.023) | 0.184 (0.004) |
| 49       | STC    | <b>0.139 (0.007)</b>  | -0.275 (0.007) | 0.553 (0.007) | 0.067 (0.003) | 0.208 (0.007) | <b>0.880 (0.010)</b> | 0.969 (0.022) | 0.218 (0.005) |
| 49       | Bucher | <b>-0.156 (0.006)</b> | -0.544 (0.006) | 0.232 (0.006) | 0.062 (0.002) | 0.201 (0.006) | <b>0.895 (0.010)</b> | 1.026 (0.023) | 0.193 (0.004) |
| 50       | MAIC   | 0.002 (0.005)         | -0.284 (0.005) | 0.288 (0.005) | 0.021 (0.001) | 0.117 (0.005) | 0.947 (0.007)        | 1.004 (0.022) | 0.145 (0.003) |
| 50       | STC    | <b>0.135 (0.005)</b>  | -0.176 (0.005) | 0.446 (0.005) | 0.045 (0.002) | 0.172 (0.005) | <b>0.856 (0.011)</b> | 0.966 (0.022) | 0.164 (0.004) |
| 50       | Bucher | <b>-0.157 (0.005)</b> | -0.455 (0.005) | 0.141 (0.005) | 0.048 (0.002) | 0.182 (0.005) | <b>0.830 (0.012)</b> | 0.996 (0.022) | 0.153 (0.003) |
| 51       | MAIC   | 0.007 (0.004)         | -0.227 (0.004) | 0.242 (0.004) | 0.013 (0.001) | 0.090 (0.004) | 0.962 (0.006)        | 1.062 (0.024) | 0.113 (0.003) |
| 51       | STC    | <b>0.139 (0.004)</b>  | -0.110 (0.004) | 0.387 (0.004) | 0.034 (0.001) | 0.153 (0.004) | <b>0.823 (0.012)</b> | 1.046 (0.023) | 0.121 (0.003) |
| 51       | Bucher | <b>-0.150 (0.004)</b> | -0.392 (0.004) | 0.092 (0.004) | 0.036 (0.001) | 0.161 (0.004) | <b>0.787 (0.013)</b> | 1.060 (0.024) | 0.117 (0.003) |
| 52       | MAIC   | 0.005 (0.006)         | -0.356 (0.006) | 0.366 (0.006) | 0.033 (0.001) | 0.147 (0.006) | 0.953 (0.007)        | 1.010 (0.023) | 0.182 (0.004) |
| 52       | STC    | 0.111 (0.007)         | -0.300 (0.007) | 0.522 (0.007) | 0.064 (0.003) | 0.202 (0.007) | <b>0.896 (0.010)</b> | 0.925 (0.021) | 0.226 (0.005) |
| 52       | Bucher | <b>-0.123 (0.006)</b> | -0.505 (0.006) | 0.258 (0.006) | 0.053 (0.002) | 0.185 (0.006) | <b>0.922 (0.008)</b> | 1.006 (0.023) | 0.193 (0.004) |
| 53       | MAIC   | 0.002 (0.004)         | -0.278 (0.004) | 0.282 (0.004) | 0.019 (0.001) | 0.109 (0.004) | 0.951 (0.007)        | 1.026 (0.023) | 0.139 (0.003) |
| 53       | STC    | <b>0.112 (0.005)</b>  | -0.196 (0.005) | 0.419 (0.005) | 0.037 (0.002) | 0.154 (0.005) | <b>0.893 (0.010)</b> | 1.007 (0.023) | 0.156 (0.003) |
| 53       | Bucher | <b>-0.127 (0.005)</b> | -0.421 (0.005) | 0.167 (0.005) | 0.038 (0.002) | 0.158 (0.005) | <b>0.866 (0.011)</b> | 1.020 (0.023) | 0.147 (0.003) |
| 54       | MAIC   | 0.000 (0.004)         | -0.230 (0.004) | 0.230 (0.003) | 0.012 (0.001) | 0.089 (0.004) | <b>0.964 (0.006)</b> | 1.061 (0.024) | 0.111 (0.002) |
| 54       | STC    | <b>0.119 (0.004)</b>  | -0.126 (0.004) | 0.365 (0.004) | 0.029 (0.001) | 0.138 (0.004) | <b>0.860 (0.011)</b> | 1.041 (0.023) | 0.120 (0.003) |
| 54       | Bucher | <b>-0.129 (0.004)</b> | -0.367 (0.004) | 0.110 (0.004) | 0.030 (0.001) | 0.143 (0.004) | <b>0.829 (0.012)</b> | 1.062 (0.024) | 0.114 (0.003) |
| 55       | MAIC   | -0.010 (0.009)        | -0.524 (0.009) | 0.505 (0.009) | 0.077 (0.003) | 0.224 (0.009) | 0.941 (0.007)        | 0.948 (0.022) | 0.277 (0.006) |
| 55       | STC    | -0.067 (0.009)        | -0.612 (0.010) | 0.478 (0.009) | 0.091 (0.004) | 0.242 (0.009) | <b>0.930 (0.008)</b> | 0.943 (0.021) | 0.295 (0.007) |
| 55       | Bucher | <b>-0.172 (0.007)</b> | -0.590 (0.007) | 0.247 (0.007) | 0.077 (0.003) | 0.222 (0.007) | <b>0.878 (0.010)</b> | 0.977 (0.022) | 0.218 (0.005) |
| 56       | MAIC   | -0.005 (0.006)        | -0.397 (0.006) | 0.387 (0.006) | 0.039 (0.002) | 0.159 (0.006) | 0.948 (0.007)        | 1.008 (0.023) | 0.198 (0.004) |
| 56       | STC    | -0.041 (0.006)        | -0.438 (0.006) | 0.356 (0.006) | 0.042 (0.002) | 0.164 (0.006) | 0.949 (0.007)        | 1.004 (0.023) | 0.202 (0.005) |
| 56       | Bucher | <b>-0.175 (0.005)</b> | -0.496 (0.005) | 0.145 (0.005) | 0.055 (0.002) | 0.196 (0.005) | <b>0.828 (0.012)</b> | 1.041 (0.023) | 0.157 (0.004) |
| 57       | MAIC   | -0.006 (0.005)        | -0.310 (0.005) | 0.299 (0.005) | 0.024 (0.001) | 0.123 (0.005) | 0.954 (0.007)        | 1.003 (0.023) | 0.155 (0.003) |
| 57       | STC    | -0.041 (0.005)        | -0.345 (0.005) | 0.263 (0.005) | 0.026 (0.001) | 0.127 (0.005) | 0.941 (0.007)        | 1.004 (0.022) | 0.155 (0.003) |
| 57       | Bucher | <b>-0.174 (0.004)</b> | -0.433 (0.004) | 0.084 (0.004) | 0.048 (0.002) | 0.186 (0.004) | <b>0.742 (0.014)</b> | 1.006 (0.023) | 0.131 (0.003) |



Table 3: Performance metrics for each method and simulation scenario. Monte Carlo standard errors for each measure are presented in parentheses. ATE: average estimated marginal treatment effect for  $A$  vs.  $B$  (is equal to the bias as the true effect is zero); LCI: average lower bound of the 95 percent confidence interval; UCI: average upper bound of the 95 percent confidence interval; MSE: mean square error; MAE: mean absolute error; Cov: coverage rate of the 95 percent confidence intervals; VR: variability ratio; ESE: empirical standard error; MAIC: matching-adjusted indirect comparison; STC: simulated treatment comparison. (*continued*)

| Scenario | Method | ATE                   | LCI            | UCI            | MSE           | MAE           | Cov                  | VR            | ESE           |
|----------|--------|-----------------------|----------------|----------------|---------------|---------------|----------------------|---------------|---------------|
| 58       | MAIC   | -0.008 (0.008)        | -0.497 (0.009) | 0.481 (0.008)  | 0.068 (0.003) | 0.208 (0.008) | 0.940 (0.008)        | 0.957 (0.022) | 0.261 (0.006) |
| 58       | STC    | -0.116 (0.009)        | -0.649 (0.009) | 0.417 (0.009)  | 0.094 (0.004) | 0.244 (0.009) | <b>0.929 (0.008)</b> | 0.960 (0.022) | 0.283 (0.006) |
| 58       | Bucher | <b>-0.164 (0.006)</b> | -0.571 (0.007) | 0.243 (0.006)  | 0.069 (0.003) | 0.209 (0.006) | <b>0.884 (0.010)</b> | 1.017 (0.023) | 0.204 (0.005) |
| 59       | MAIC   | 0.000 (0.006)         | -0.370 (0.006) | 0.370 (0.006)  | 0.036 (0.002) | 0.150 (0.006) | 0.948 (0.007)        | 0.999 (0.023) | 0.189 (0.004) |
| 59       | STC    | -0.091 (0.006)        | -0.478 (0.007) | 0.297 (0.006)  | 0.049 (0.002) | 0.175 (0.006) | <b>0.919 (0.009)</b> | 0.976 (0.022) | 0.203 (0.005) |
| 59       | Bucher | <b>-0.154 (0.005)</b> | -0.465 (0.005) | 0.157 (0.005)  | 0.050 (0.002) | 0.183 (0.005) | <b>0.839 (0.012)</b> | 0.976 (0.022) | 0.163 (0.004) |
| 60       | MAIC   | 0.002 (0.005)         | -0.288 (0.005) | 0.292 (0.005)  | 0.022 (0.001) | 0.117 (0.005) | 0.949 (0.007)        | 0.998 (0.022) | 0.148 (0.003) |
| 60       | STC    | <b>-0.086 (0.005)</b> | -0.383 (0.005) | 0.212 (0.005)  | 0.031 (0.001) | 0.141 (0.005) | <b>0.907 (0.009)</b> | 0.986 (0.022) | 0.154 (0.003) |
| 60       | Bucher | <b>-0.158 (0.004)</b> | -0.409 (0.004) | 0.094 (0.004)  | 0.042 (0.002) | 0.171 (0.004) | <b>0.763 (0.013)</b> | 0.971 (0.022) | 0.132 (0.003) |
| 61       | MAIC   | 0.000 (0.008)         | -0.464 (0.008) | 0.463 (0.008)  | 0.064 (0.003) | 0.201 (0.008) | <b>0.926 (0.008)</b> | 0.936 (0.021) | 0.253 (0.006) |
| 61       | STC    | <b>-0.187 (0.009)</b> | -0.712 (0.009) | 0.338 (0.009)  | 0.115 (0.005) | 0.268 (0.009) | <b>0.885 (0.010)</b> | 0.949 (0.021) | 0.283 (0.006) |
| 61       | Bucher | <b>-0.143 (0.007)</b> | -0.538 (0.007) | 0.253 (0.006)  | 0.064 (0.003) | 0.202 (0.007) | <b>0.893 (0.010)</b> | 0.968 (0.022) | 0.209 (0.005) |
| 62       | MAIC   | -0.005 (0.006)        | -0.356 (0.006) | 0.345 (0.006)  | 0.034 (0.001) | 0.148 (0.006) | <b>0.932 (0.008)</b> | 0.972 (0.022) | 0.184 (0.004) |
| 62       | STC    | <b>-0.178 (0.006)</b> | -0.559 (0.006) | 0.202 (0.006)  | 0.072 (0.003) | 0.215 (0.006) | <b>0.848 (0.011)</b> | 0.965 (0.022) | 0.201 (0.004) |
| 62       | Bucher | <b>-0.137 (0.005)</b> | -0.440 (0.005) | 0.165 (0.005)  | 0.045 (0.002) | 0.172 (0.005) | <b>0.839 (0.012)</b> | 0.948 (0.021) | 0.163 (0.004) |
| 63       | MAIC   | -0.007 (0.004)        | -0.283 (0.004) | 0.270 (0.005)  | 0.020 (0.001) | 0.113 (0.004) | 0.952 (0.007)        | 0.998 (0.022) | 0.141 (0.003) |
| 63       | STC    | <b>-0.170 (0.005)</b> | -0.462 (0.005) | 0.121 (0.005)  | 0.052 (0.002) | 0.187 (0.005) | <b>0.794 (0.013)</b> | 0.986 (0.022) | 0.151 (0.003) |
| 63       | Bucher | <b>-0.142 (0.004)</b> | -0.386 (0.004) | 0.103 (0.004)  | 0.036 (0.001) | 0.156 (0.004) | <b>0.804 (0.013)</b> | 1.000 (0.022) | 0.125 (0.003) |
| 64       | MAIC   | 0.008 (0.008)         | -0.484 (0.009) | 0.501 (0.009)  | 0.072 (0.003) | 0.210 (0.008) | <b>0.924 (0.008)</b> | 0.939 (0.021) | 0.268 (0.006) |
| 64       | STC    | 0.008 (0.009)         | -0.525 (0.009) | 0.542 (0.009)  | 0.082 (0.004) | 0.226 (0.009) | <b>0.931 (0.008)</b> | 0.951 (0.021) | 0.286 (0.006) |
| 64       | Bucher | <b>-0.270 (0.007)</b> | -0.680 (0.007) | 0.139 (0.006)  | 0.118 (0.004) | 0.289 (0.007) | <b>0.742 (0.014)</b> | 0.990 (0.022) | 0.211 (0.005) |
| 65       | MAIC   | -0.001 (0.006)        | -0.374 (0.006) | 0.371 (0.006)  | 0.038 (0.002) | 0.155 (0.006) | <b>0.933 (0.008)</b> | 0.975 (0.022) | 0.195 (0.004) |
| 65       | STC    | 0.000 (0.006)         | -0.387 (0.007) | 0.387 (0.006)  | 0.041 (0.002) | 0.162 (0.006) | 0.941 (0.007)        | 0.969 (0.022) | 0.204 (0.005) |
| 65       | Bucher | <b>-0.275 (0.005)</b> | -0.589 (0.005) | 0.039 (0.005)  | 0.102 (0.003) | 0.282 (0.005) | <b>0.593 (0.016)</b> | 0.995 (0.022) | 0.161 (0.004) |
| 66       | MAIC   | -0.003 (0.005)        | -0.297 (0.005) | 0.291 (0.005)  | 0.024 (0.001) | 0.123 (0.005) | 0.937 (0.008)        | 0.970 (0.022) | 0.155 (0.003) |
| 66       | STC    | 0.002 (0.005)         | -0.296 (0.005) | 0.300 (0.005)  | 0.024 (0.001) | 0.124 (0.005) | 0.937 (0.008)        | 0.972 (0.022) | 0.156 (0.003) |
| 66       | Bucher | <b>-0.286 (0.004)</b> | -0.539 (0.004) | -0.032 (0.004) | 0.099 (0.003) | 0.287 (0.004) | <b>0.414 (0.016)</b> | 0.974 (0.022) | 0.133 (0.003) |
| 67       | MAIC   | -0.016 (0.008)        | -0.487 (0.008) | 0.455 (0.008)  | 0.062 (0.003) | 0.197 (0.008) | <b>0.931 (0.008)</b> | 0.965 (0.022) | 0.249 (0.006) |
| 67       | STC    | -0.047 (0.009)        | -0.572 (0.009) | 0.478 (0.009)  | 0.077 (0.003) | 0.222 (0.009) | 0.952 (0.007)        | 0.978 (0.022) | 0.274 (0.006) |
| 67       | Bucher | <b>-0.260 (0.006)</b> | -0.661 (0.007) | 0.142 (0.006)  | 0.108 (0.004) | 0.278 (0.006) | <b>0.766 (0.013)</b> | 1.012 (0.023) | 0.203 (0.005) |
| 68       | MAIC   | -0.005 (0.006)        | -0.363 (0.006) | 0.353 (0.006)  | 0.034 (0.002) | 0.147 (0.006) | 0.956 (0.006)        | 0.995 (0.022) | 0.183 (0.004) |
| 68       | STC    | -0.030 (0.006)        | -0.411 (0.006) | 0.351 (0.006)  | 0.038 (0.002) | 0.154 (0.006) | 0.950 (0.007)        | 1.015 (0.023) | 0.191 (0.004) |
| 68       | Bucher | <b>-0.258 (0.005)</b> | -0.566 (0.005) | 0.049 (0.005)  | 0.090 (0.003) | 0.265 (0.005) | <b>0.622 (0.015)</b> | 1.024 (0.023) | 0.153 (0.003) |
| 69       | MAIC   | 0.006 (0.004)         | -0.276 (0.004) | 0.288 (0.004)  | 0.019 (0.001) | 0.109 (0.004) | 0.958 (0.006)        | 1.045 (0.023) | 0.138 (0.003) |
| 69       | STC    | -0.015 (0.005)        | -0.307 (0.005) | 0.277 (0.005)  | 0.022 (0.001) | 0.118 (0.005) | 0.956 (0.006)        | 1.016 (0.023) | 0.147 (0.003) |
| 69       | Bucher | <b>-0.247 (0.004)</b> | -0.495 (0.004) | 0.001 (0.004)  | 0.077 (0.002) | 0.249 (0.004) | <b>0.517 (0.016)</b> | 1.019 (0.023) | 0.124 (0.003) |
| 70       | MAIC   | -0.009 (0.007)        | -0.458 (0.007) | 0.440 (0.008)  | 0.054 (0.002) | 0.186 (0.007) | 0.943 (0.007)        | 0.983 (0.022) | 0.233 (0.005) |
| 70       | STC    | -0.083 (0.009)        | -0.598 (0.009) | 0.431 (0.008)  | 0.080 (0.004) | 0.224 (0.009) | <b>0.934 (0.008)</b> | 0.969 (0.022) | 0.271 (0.006) |
| 70       | Bucher | <b>-0.216 (0.006)</b> | -0.607 (0.006) | 0.176 (0.006)  | 0.086 (0.003) | 0.244 (0.006) | <b>0.825 (0.012)</b> | 1.008 (0.023) | 0.198 (0.004) |
| 71       | MAIC   | 0.005 (0.006)         | -0.338 (0.006) | 0.348 (0.006)  | 0.033 (0.001) | 0.144 (0.006) | <b>0.933 (0.008)</b> | 0.963 (0.022) | 0.182 (0.004) |
| 71       | STC    | -0.065 (0.006)        | -0.440 (0.006) | 0.309 (0.006)  | 0.041 (0.002) | 0.164 (0.006) | <b>0.935 (0.008)</b> | 0.994 (0.022) | 0.192 (0.004) |
| 71       | Bucher | <b>-0.218 (0.005)</b> | -0.518 (0.005) | 0.083 (0.005)  | 0.071 (0.002) | 0.229 (0.005) | <b>0.701 (0.014)</b> | 0.986 (0.022) | 0.155 (0.003) |
| 72       | MAIC   | 0.008 (0.004)         | -0.264 (0.004) | 0.279 (0.004)  | 0.019 (0.001) | 0.111 (0.004) | 0.952 (0.007)        | 1.002 (0.022) | 0.138 (0.003) |
| 72       | STC    | -0.054 (0.005)        | -0.340 (0.005) | 0.233 (0.005)  | 0.025 (0.001) | 0.125 (0.005) | <b>0.930 (0.008)</b> | 0.979 (0.022) | 0.149 (0.003) |
| 72       | Bucher | <b>-0.210 (0.004)</b> | -0.453 (0.004) | 0.032 (0.004)  | 0.060 (0.002) | 0.214 (0.004) | <b>0.606 (0.015)</b> | 0.977 (0.022) | 0.127 (0.003) |
| 73       | MAIC   | 0.001 (0.008)         | -0.468 (0.008) | 0.469 (0.008)  | 0.065 (0.003) | 0.205 (0.008) | <b>0.931 (0.008)</b> | 0.938 (0.021) | 0.255 (0.006) |
| 73       | STC    | 0.108 (0.009)         | -0.417 (0.009) | 0.632 (0.009)  | 0.094 (0.004) | 0.246 (0.009) | <b>0.910 (0.009)</b> | 0.933 (0.021) | 0.287 (0.006) |
| 73       | Bucher | <b>-0.413 (0.006)</b> | -0.816 (0.007) | -0.010 (0.006) | 0.211 (0.006) | 0.414 (0.006) | <b>0.486 (0.016)</b> | 1.018 (0.023) | 0.202 (0.005) |
| 74       | MAIC   | 0.018 (0.006)         | -0.339 (0.006) | 0.376 (0.006)  | 0.031 (0.002) | 0.140 (0.006) | 0.954 (0.007)        | 1.035 (0.023) | 0.176 (0.004) |
| 74       | STC    | <b>0.113 (0.006)</b>  | -0.268 (0.006) | 0.493 (0.006)  | 0.050 (0.002) | 0.176 (0.006) | <b>0.910 (0.009)</b> | 1.005 (0.023) | 0.193 (0.004) |
| 74       | Bucher | <b>-0.399 (0.005)</b> | -0.708 (0.005) | -0.091 (0.005) | 0.184 (0.004) | 0.400 (0.005) | <b>0.276 (0.014)</b> | 0.993 (0.022) | 0.158 (0.004) |
| 75       | MAIC   | 0.006 (0.004)         | -0.275 (0.004) | 0.287 (0.004)  | 0.020 (0.001) | 0.112 (0.004) | 0.956 (0.006)        | 1.025 (0.023) | 0.140 (0.003) |
| 75       | STC    | <b>0.105 (0.005)</b>  | -0.187 (0.005) | 0.398 (0.005)  | 0.033 (0.001) | 0.148 (0.005) | <b>0.898 (0.010)</b> | 1.010 (0.023) | 0.148 (0.003) |
| 75       | Bucher | <b>-0.405 (0.004)</b> | -0.654 (0.004) | -0.156 (0.004) | 0.180 (0.003) | 0.405 (0.004) | <b>0.110 (0.010)</b> | 0.995 (0.022) | 0.128 (0.003) |
| 76       | MAIC   | 0.011 (0.008)         | -0.444 (0.008) | 0.466 (0.008)  | 0.059 (0.003) | 0.193 (0.008) | <b>0.936 (0.008)</b> | 0.955 (0.022) | 0.243 (0.005) |
| 76       | STC    | 0.111 (0.009)         | -0.405 (0.009) | 0.628 (0.009)  | 0.089 (0.004) | 0.237 (0.009) | <b>0.922 (0.008)</b> | 0.951 (0.021) | 0.277 (0.006) |
| 76       | Bucher | <b>-0.364 (0.006)</b> | -0.760 (0.006) | 0.033 (0.006)  | 0.172 (0.005) | 0.369 (0.006) | <b>0.564 (0.016)</b> | 1.013 (0.023) | 0.200 (0.004) |
| 77       | MAIC   | 0.016 (0.005)         | -0.330 (0.006) | 0.363 (0.005)  | 0.030 (0.001) | 0.139 (0.005) | 0.947 (0.007)        | 1.019 (0.023) | 0.173 (0.004) |
| 77       | STC    | <b>0.119 (0.006)</b>  | -0.257 (0.006) | 0.495 (0.006)  | 0.051 (0.002) | 0.182 (0.006) | <b>0.904 (0.009)</b> | 0.996 (0.022) | 0.192 (0.004) |
| 77       | Bucher | <b>-0.367 (0.005)</b> | -0.670 (0.005) | -0.063 (0.005) | 0.158 (0.004) | 0.367 (0.005) | <b>0.324 (0.015)</b> | 1.015 (0.023) | 0.153 (0.003) |

Table 3: Performance metrics for each method and simulation scenario. Monte Carlo standard errors for each measure are presented in parentheses. ATE: average estimated marginal treatment effect for  $A$  vs.  $B$  (is equal to the bias as the true effect is zero); LCI: average lower bound of the 95 percent confidence interval; UCI: average upper bound of the 95 percent confidence interval; MSE: mean square error; MAE: mean absolute error; Cov: coverage rate of the 95 percent confidence intervals; VR: variability ratio; ESE: empirical standard error; MAIC: matching-adjusted indirect comparison; STC: simulated treatment comparison. (*continued*)

| Scenario | Method | ATE                   | LCI            | UCI            | MSE           | MAE           | Cov                  | VR            | ESE           |
|----------|--------|-----------------------|----------------|----------------|---------------|---------------|----------------------|---------------|---------------|
| 78       | MAIC   | 0.013 (0.004)         | -0.261 (0.004) | 0.287 (0.004)  | 0.019 (0.001) | 0.109 (0.004) | 0.951 (0.007)        | 1.023 (0.023) | 0.137 (0.003) |
| 78       | STC    | <b>0.123 (0.005)</b>  | -0.165 (0.005) | 0.411 (0.005)  | 0.038 (0.002) | 0.157 (0.005) | <b>0.859 (0.011)</b> | 0.973 (0.022) | 0.151 (0.003) |
| 78       | Bucher | <b>-0.367 (0.004)</b> | -0.612 (0.004) | -0.122 (0.004) | 0.150 (0.003) | 0.367 (0.004) | <b>0.158 (0.012)</b> | 1.002 (0.022) | 0.125 (0.003) |
| 79       | MAIC   | 0.008 (0.007)         | -0.431 (0.007) | 0.447 (0.007)  | 0.052 (0.002) | 0.182 (0.007) | 0.942 (0.007)        | 0.986 (0.022) | 0.227 (0.005) |
| 79       | STC    | 0.110 (0.008)         | -0.400 (0.008) | 0.620 (0.008)  | 0.081 (0.004) | 0.226 (0.008) | <b>0.926 (0.008)</b> | 0.992 (0.022) | 0.263 (0.006) |
| 79       | Bucher | <b>-0.321 (0.006)</b> | -0.710 (0.006) | 0.068 (0.006)  | 0.141 (0.004) | 0.328 (0.006) | <b>0.645 (0.015)</b> | 1.010 (0.023) | 0.197 (0.004) |
| 80       | MAIC   | 0.012 (0.005)         | -0.325 (0.005) | 0.348 (0.005)  | 0.029 (0.001) | 0.137 (0.005) | 0.944 (0.007)        | 1.007 (0.023) | 0.170 (0.004) |
| 80       | STC    | <b>0.113 (0.006)</b>  | -0.257 (0.006) | 0.483 (0.006)  | 0.050 (0.002) | 0.177 (0.006) | <b>0.901 (0.009)</b> | 0.979 (0.022) | 0.193 (0.004) |
| 80       | Bucher | <b>-0.313 (0.005)</b> | -0.611 (0.005) | -0.015 (0.005) | 0.120 (0.003) | 0.314 (0.005) | <b>0.442 (0.016)</b> | 1.023 (0.023) | 0.149 (0.003) |
| 81       | MAIC   | 0.003 (0.004)         | -0.264 (0.004) | 0.270 (0.004)  | 0.018 (0.001) | 0.108 (0.004) | 0.961 (0.006)        | 1.023 (0.023) | 0.133 (0.003) |
| 81       | STC    | <b>0.106 (0.004)</b>  | -0.179 (0.004) | 0.390 (0.005)  | 0.031 (0.001) | 0.143 (0.004) | <b>0.900 (0.009)</b> | 1.022 (0.023) | 0.142 (0.003) |
| 81       | Bucher | <b>-0.324 (0.004)</b> | -0.564 (0.004) | -0.083 (0.004) | 0.120 (0.003) | 0.324 (0.004) | <b>0.245 (0.014)</b> | 1.012 (0.023) | 0.121 (0.003) |
| 82       | MAIC   | 0.006 (0.008)         | -0.461 (0.008) | 0.473 (0.007)  | 0.057 (0.003) | 0.192 (0.008) | 0.948 (0.007)        | 0.997 (0.022) | 0.239 (0.005) |
| 82       | STC    | -0.070 (0.008)        | -0.583 (0.009) | 0.442 (0.008)  | 0.077 (0.004) | 0.218 (0.008) | 0.937 (0.008)        | 0.973 (0.022) | 0.268 (0.006) |
| 82       | Bucher | <b>-0.163 (0.007)</b> | -0.581 (0.007) | 0.254 (0.006)  | 0.071 (0.003) | 0.214 (0.007) | <b>0.888 (0.010)</b> | 1.011 (0.023) | 0.210 (0.005) |
| 83       | MAIC   | 0.001 (0.006)         | -0.352 (0.006) | 0.354 (0.006)  | 0.035 (0.002) | 0.150 (0.006) | 0.945 (0.007)        | 0.958 (0.022) | 0.188 (0.004) |
| 83       | STC    | -0.063 (0.006)        | -0.437 (0.006) | 0.311 (0.006)  | 0.043 (0.002) | 0.166 (0.006) | <b>0.936 (0.008)</b> | 0.968 (0.022) | 0.197 (0.004) |
| 83       | Bucher | <b>-0.158 (0.005)</b> | -0.477 (0.005) | 0.161 (0.005)  | 0.054 (0.002) | 0.191 (0.005) | <b>0.836 (0.012)</b> | 0.959 (0.021) | 0.170 (0.004) |
| 84       | MAIC   | -0.005 (0.004)        | -0.285 (0.004) | 0.276 (0.004)  | 0.020 (0.001) | 0.111 (0.004) | 0.948 (0.007)        | 1.013 (0.023) | 0.141 (0.003) |
| 84       | STC    | -0.066 (0.005)        | -0.356 (0.005) | 0.225 (0.005)  | 0.026 (0.001) | 0.130 (0.005) | <b>0.932 (0.008)</b> | 1.005 (0.022) | 0.147 (0.003) |
| 84       | Bucher | <b>-0.159 (0.004)</b> | -0.417 (0.004) | 0.098 (0.004)  | 0.043 (0.002) | 0.175 (0.004) | <b>0.781 (0.013)</b> | 0.990 (0.022) | 0.133 (0.003) |
| 85       | MAIC   | 0.004 (0.007)         | -0.434 (0.007) | 0.443 (0.007)  | 0.050 (0.003) | 0.175 (0.007) | 0.951 (0.007)        | 1.000 (0.023) | 0.224 (0.005) |
| 85       | STC    | <b>-0.158 (0.008)</b> | -0.658 (0.009) | 0.343 (0.008)  | 0.094 (0.004) | 0.244 (0.008) | <b>0.901 (0.009)</b> | 0.969 (0.022) | 0.264 (0.006) |
| 85       | Bucher | <b>-0.132 (0.007)</b> | -0.537 (0.007) | 0.274 (0.006)  | 0.061 (0.003) | 0.197 (0.007) | <b>0.918 (0.009)</b> | 0.989 (0.022) | 0.209 (0.005) |
| 86       | MAIC   | 0.007 (0.005)         | -0.328 (0.005) | 0.342 (0.005)  | 0.027 (0.001) | 0.132 (0.005) | 0.951 (0.007)        | 1.035 (0.023) | 0.165 (0.004) |
| 86       | STC    | <b>-0.145 (0.006)</b> | -0.510 (0.006) | 0.221 (0.006)  | 0.055 (0.002) | 0.188 (0.006) | <b>0.880 (0.010)</b> | 1.006 (0.023) | 0.186 (0.004) |
| 86       | Bucher | <b>-0.138 (0.005)</b> | -0.448 (0.005) | 0.173 (0.005)  | 0.043 (0.002) | 0.169 (0.005) | <b>0.869 (0.011)</b> | 1.025 (0.023) | 0.154 (0.003) |
| 87       | MAIC   | 0.006 (0.004)         | -0.261 (0.004) | 0.273 (0.004)  | 0.017 (0.001) | 0.104 (0.004) | 0.957 (0.006)        | 1.046 (0.023) | 0.130 (0.003) |
| 87       | STC    | <b>-0.137 (0.004)</b> | -0.420 (0.004) | 0.147 (0.004)  | 0.038 (0.001) | 0.162 (0.004) | <b>0.849 (0.011)</b> | 1.033 (0.023) | 0.140 (0.003) |
| 87       | Bucher | <b>-0.136 (0.004)</b> | -0.386 (0.004) | 0.115 (0.004)  | 0.033 (0.001) | 0.152 (0.004) | <b>0.828 (0.012)</b> | 1.044 (0.023) | 0.123 (0.003) |
| 88       | MAIC   | 0.019 (0.007)         | -0.397 (0.007) | 0.435 (0.007)  | 0.049 (0.002) | 0.179 (0.007) | 0.942 (0.007)        | 0.965 (0.022) | 0.220 (0.005) |
| 88       | STC    | <b>-0.250 (0.008)</b> | -0.741 (0.008) | 0.242 (0.008)  | 0.129 (0.005) | 0.292 (0.008) | <b>0.826 (0.012)</b> | 0.972 (0.022) | 0.258 (0.006) |
| 88       | Bucher | -0.104 (0.007)        | -0.499 (0.007) | 0.291 (0.007)  | 0.056 (0.003) | 0.188 (0.007) | <b>0.918 (0.009)</b> | 0.945 (0.021) | 0.213 (0.005) |
| 89       | MAIC   | -0.001 (0.005)        | -0.322 (0.005) | 0.320 (0.005)  | 0.027 (0.001) | 0.128 (0.005) | 0.938 (0.008)        | 1.005 (0.023) | 0.163 (0.004) |
| 89       | STC    | <b>-0.245 (0.006)</b> | -0.605 (0.006) | 0.115 (0.006)  | 0.095 (0.003) | 0.261 (0.006) | <b>0.747 (0.014)</b> | 0.989 (0.022) | 0.186 (0.004) |
| 89       | Bucher | <b>-0.112 (0.005)</b> | -0.414 (0.005) | 0.191 (0.005)  | 0.038 (0.002) | 0.157 (0.005) | <b>0.884 (0.010)</b> | 0.975 (0.022) | 0.158 (0.004) |
| 90       | MAIC   | 0.003 (0.004)         | -0.254 (0.004) | 0.260 (0.004)  | 0.017 (0.001) | 0.106 (0.004) | 0.949 (0.007)        | 0.995 (0.022) | 0.132 (0.003) |
| 90       | STC    | <b>-0.240 (0.004)</b> | -0.518 (0.004) | 0.039 (0.004)  | 0.077 (0.002) | 0.244 (0.004) | <b>0.603 (0.015)</b> | 1.029 (0.023) | 0.138 (0.003) |
| 90       | Bucher | <b>-0.111 (0.004)</b> | -0.356 (0.004) | 0.133 (0.004)  | 0.028 (0.001) | 0.136 (0.004) | <b>0.850 (0.011)</b> | 0.994 (0.022) | 0.126 (0.003) |
| 91       | MAIC   | -0.002 (0.007)        | -0.450 (0.008) | 0.447 (0.007)  | 0.055 (0.003) | 0.187 (0.007) | 0.938 (0.008)        | 0.978 (0.022) | 0.234 (0.005) |
| 91       | STC    | -0.007 (0.008)        | -0.506 (0.009) | 0.493 (0.008)  | 0.071 (0.003) | 0.213 (0.008) | 0.945 (0.007)        | 0.958 (0.022) | 0.266 (0.006) |
| 91       | Bucher | <b>-0.247 (0.007)</b> | -0.658 (0.007) | 0.163 (0.006)  | 0.105 (0.004) | 0.272 (0.007) | <b>0.790 (0.013)</b> | 0.996 (0.022) | 0.210 (0.005) |
| 92       | MAIC   | -0.005 (0.006)        | -0.347 (0.006) | 0.337 (0.005)  | 0.030 (0.001) | 0.138 (0.006) | 0.946 (0.007)        | 1.001 (0.022) | 0.174 (0.004) |
| 92       | STC    | -0.007 (0.006)        | -0.374 (0.006) | 0.359 (0.006)  | 0.037 (0.002) | 0.153 (0.006) | 0.941 (0.007)        | 0.976 (0.022) | 0.192 (0.004) |
| 92       | Bucher | <b>-0.256 (0.005)</b> | -0.571 (0.005) | 0.058 (0.005)  | 0.092 (0.003) | 0.262 (0.005) | <b>0.648 (0.015)</b> | 0.984 (0.022) | 0.163 (0.004) |
| 93       | MAIC   | -0.002 (0.004)        | -0.274 (0.004) | 0.270 (0.004)  | 0.018 (0.001) | 0.107 (0.004) | 0.959 (0.006)        | 1.024 (0.023) | 0.136 (0.003) |
| 93       | STC    | -0.004 (0.005)        | -0.289 (0.005) | 0.281 (0.005)  | 0.021 (0.001) | 0.114 (0.005) | 0.953 (0.007)        | 1.011 (0.023) | 0.144 (0.003) |
| 93       | Bucher | <b>-0.258 (0.004)</b> | -0.512 (0.004) | -0.004 (0.004) | 0.083 (0.002) | 0.261 (0.004) | <b>0.469 (0.016)</b> | 1.016 (0.023) | 0.128 (0.003) |
| 94       | MAIC   | 0.003 (0.007)         | -0.428 (0.007) | 0.434 (0.007)  | 0.051 (0.002) | 0.180 (0.007) | 0.942 (0.007)        | 0.974 (0.022) | 0.226 (0.005) |
| 94       | STC    | -0.043 (0.008)        | -0.536 (0.009) | 0.451 (0.008)  | 0.072 (0.004) | 0.211 (0.008) | <b>0.932 (0.008)</b> | 0.949 (0.021) | 0.265 (0.006) |
| 94       | Bucher | <b>-0.218 (0.007)</b> | -0.620 (0.007) | 0.184 (0.006)  | 0.091 (0.004) | 0.249 (0.007) | <b>0.823 (0.012)</b> | 0.981 (0.022) | 0.209 (0.005) |
| 95       | MAIC   | 0.005 (0.005)         | -0.324 (0.006) | 0.333 (0.005)  | 0.030 (0.001) | 0.138 (0.005) | 0.949 (0.007)        | 0.970 (0.022) | 0.173 (0.004) |
| 95       | STC    | -0.039 (0.006)        | -0.399 (0.006) | 0.321 (0.006)  | 0.038 (0.002) | 0.153 (0.006) | 0.937 (0.008)        | 0.964 (0.022) | 0.191 (0.004) |
| 95       | Bucher | <b>-0.213 (0.005)</b> | -0.521 (0.005) | 0.094 (0.005)  | 0.071 (0.002) | 0.226 (0.005) | <b>0.710 (0.014)</b> | 0.985 (0.022) | 0.159 (0.004) |
| 96       | MAIC   | -0.003 (0.004)        | -0.266 (0.004) | 0.261 (0.004)  | 0.016 (0.001) | 0.103 (0.004) | 0.962 (0.006)        | 1.049 (0.023) | 0.128 (0.003) |
| 96       | STC    | -0.047 (0.004)        | -0.327 (0.004) | 0.233 (0.004)  | 0.022 (0.001) | 0.118 (0.004) | <b>0.935 (0.008)</b> | 1.012 (0.023) | 0.141 (0.003) |
| 96       | Bucher | <b>-0.222 (0.004)</b> | -0.471 (0.004) | 0.026 (0.004)  | 0.065 (0.002) | 0.225 (0.004) | <b>0.587 (0.016)</b> | 1.023 (0.023) | 0.124 (0.003) |
| 97       | MAIC   | -0.008 (0.007)        | -0.423 (0.007) | 0.406 (0.007)  | 0.048 (0.002) | 0.172 (0.007) | <b>0.928 (0.008)</b> | 0.967 (0.022) | 0.219 (0.005) |
| 97       | STC    | -0.121 (0.008)        | -0.608 (0.008) | 0.367 (0.008)  | 0.076 (0.004) | 0.220 (0.008) | <b>0.931 (0.008)</b> | 1.000 (0.022) | 0.249 (0.006) |
| 97       | Bucher | <b>-0.183 (0.006)</b> | -0.576 (0.007) | 0.211 (0.006)  | 0.075 (0.003) | 0.222 (0.006) | <b>0.847 (0.011)</b> | 0.980 (0.022) | 0.205 (0.005) |

Table 3: Performance metrics for each method and simulation scenario. Monte Carlo standard errors for each measure are presented in parentheses. ATE: average estimated marginal treatment effect for  $A$  vs.  $B$  (is equal to the bias as the true effect is zero); LCI: average lower bound of the 95 percent confidence interval; UCI: average upper bound of the 95 percent confidence interval; MSE: mean square error; MAE: mean absolute error; Cov: coverage rate of the 95 percent confidence intervals; VR: variability ratio; ESE: empirical standard error; MAIC: matching-adjusted indirect comparison; STC: simulated treatment comparison. (*continued*)

| Scenario | Method | ATE                   | LCI            | UCI            | MSE           | MAE           | Cov                  | VR            | ESE           |
|----------|--------|-----------------------|----------------|----------------|---------------|---------------|----------------------|---------------|---------------|
| 98       | MAIC   | 0.015 (0.005)         | -0.305 (0.005) | 0.335 (0.005)  | 0.027 (0.001) | 0.133 (0.005) | 0.953 (0.007)        | 0.994 (0.022) | 0.164 (0.004) |
| 98       | STC    | -0.088 (0.006)        | -0.443 (0.006) | 0.268 (0.006)  | 0.042 (0.002) | 0.162 (0.006) | <b>0.925 (0.008)</b> | 0.980 (0.022) | 0.185 (0.004) |
| 98       | Bucher | <b>-0.174 (0.005)</b> | -0.476 (0.005) | 0.127 (0.005)  | 0.054 (0.002) | 0.194 (0.005) | <b>0.811 (0.012)</b> | 0.992 (0.022) | 0.155 (0.003) |
| 99       | MAIC   | 0.006 (0.004)         | -0.250 (0.004) | 0.262 (0.004)  | 0.017 (0.001) | 0.105 (0.004) | 0.960 (0.006)        | 0.997 (0.022) | 0.131 (0.003) |
| 99       | STC    | <b>-0.105 (0.004)</b> | -0.380 (0.004) | 0.171 (0.004)  | 0.030 (0.001) | 0.140 (0.004) | <b>0.882 (0.010)</b> | 1.014 (0.023) | 0.138 (0.003) |
| 99       | Bucher | <b>-0.173 (0.004)</b> | -0.416 (0.004) | 0.071 (0.004)  | 0.044 (0.001) | 0.180 (0.004) | <b>0.713 (0.014)</b> | 1.032 (0.023) | 0.120 (0.003) |
| 100      | MAIC   | -0.012 (0.007)        | -0.445 (0.007) | 0.422 (0.007)  | 0.047 (0.002) | 0.171 (0.007) | 0.951 (0.007)        | 1.023 (0.023) | 0.216 (0.005) |
| 100      | STC    | 0.108 (0.008)         | -0.385 (0.008) | 0.600 (0.008)  | 0.074 (0.003) | 0.214 (0.008) | <b>0.922 (0.008)</b> | 1.007 (0.023) | 0.250 (0.006) |
| 100      | Bucher | <b>-0.373 (0.006)</b> | -0.778 (0.006) | 0.033 (0.006)  | 0.176 (0.005) | 0.376 (0.006) | <b>0.576 (0.016)</b> | 1.072 (0.024) | 0.193 (0.004) |
| 101      | MAIC   | 0.004 (0.005)         | -0.326 (0.005) | 0.335 (0.005)  | 0.029 (0.001) | 0.136 (0.005) | 0.943 (0.007)        | 0.992 (0.022) | 0.170 (0.004) |
| 101      | STC    | <b>0.133 (0.006)</b>  | -0.227 (0.006) | 0.494 (0.006)  | 0.055 (0.002) | 0.188 (0.006) | <b>0.869 (0.011)</b> | 0.958 (0.021) | 0.192 (0.004) |
| 101      | Bucher | <b>-0.366 (0.005)</b> | -0.676 (0.005) | -0.056 (0.005) | 0.159 (0.004) | 0.367 (0.005) | <b>0.367 (0.015)</b> | 1.007 (0.023) | 0.157 (0.004) |
| 102      | MAIC   | 0.008 (0.004)         | -0.257 (0.004) | 0.272 (0.004)  | 0.016 (0.001) | 0.102 (0.004) | <b>0.965 (0.006)</b> | 1.058 (0.024) | 0.128 (0.003) |
| 102      | STC    | <b>0.133 (0.005)</b>  | -0.147 (0.005) | 0.414 (0.005)  | 0.038 (0.001) | 0.160 (0.005) | <b>0.838 (0.012)</b> | 1.003 (0.022) | 0.143 (0.003) |
| 102      | Bucher | <b>-0.366 (0.004)</b> | -0.617 (0.004) | -0.116 (0.004) | 0.149 (0.003) | 0.366 (0.004) | <b>0.176 (0.012)</b> | 1.033 (0.023) | 0.124 (0.003) |
| 103      | MAIC   | 0.005 (0.007)         | -0.414 (0.007) | 0.425 (0.007)  | 0.045 (0.002) | 0.168 (0.007) | 0.948 (0.007)        | 1.004 (0.023) | 0.213 (0.005) |
| 103      | STC    | <b>0.134 (0.008)</b>  | -0.352 (0.008) | 0.621 (0.008)  | 0.085 (0.004) | 0.230 (0.008) | <b>0.896 (0.010)</b> | 0.960 (0.022) | 0.259 (0.006) |
| 103      | Bucher | <b>-0.315 (0.006)</b> | -0.714 (0.006) | 0.084 (0.006)  | 0.139 (0.004) | 0.327 (0.006) | <b>0.653 (0.015)</b> | 1.022 (0.023) | 0.199 (0.004) |
| 104      | MAIC   | 0.002 (0.005)         | -0.320 (0.005) | 0.324 (0.005)  | 0.027 (0.001) | 0.131 (0.005) | 0.954 (0.007)        | 1.003 (0.022) | 0.164 (0.004) |
| 104      | STC    | <b>0.135 (0.006)</b>  | -0.221 (0.006) | 0.491 (0.006)  | 0.051 (0.002) | 0.181 (0.006) | <b>0.888 (0.010)</b> | 1.004 (0.022) | 0.181 (0.004) |
| 104      | Bucher | <b>-0.314 (0.005)</b> | -0.620 (0.005) | -0.009 (0.005) | 0.122 (0.003) | 0.316 (0.005) | <b>0.472 (0.016)</b> | 1.019 (0.023) | 0.153 (0.003) |
| 105      | MAIC   | 0.001 (0.004)         | -0.257 (0.004) | 0.259 (0.004)  | 0.017 (0.001) | 0.106 (0.004) | 0.958 (0.006)        | 1.005 (0.022) | 0.131 (0.003) |
| 105      | STC    | <b>0.133 (0.005)</b>  | -0.143 (0.004) | 0.409 (0.005)  | 0.038 (0.001) | 0.160 (0.005) | <b>0.836 (0.012)</b> | 0.986 (0.022) | 0.143 (0.003) |
| 105      | Bucher | <b>-0.321 (0.004)</b> | -0.568 (0.004) | -0.075 (0.004) | 0.119 (0.003) | 0.322 (0.004) | <b>0.276 (0.014)</b> | 0.986 (0.022) | 0.128 (0.003) |
| 106      | MAIC   | -0.009 (0.007)        | -0.418 (0.007) | 0.400 (0.007)  | 0.045 (0.002) | 0.169 (0.007) | 0.938 (0.008)        | 0.979 (0.022) | 0.213 (0.005) |
| 106      | STC    | 0.111 (0.008)         | -0.372 (0.008) | 0.594 (0.008)  | 0.076 (0.003) | 0.220 (0.008) | <b>0.921 (0.009)</b> | 0.976 (0.022) | 0.252 (0.006) |
| 106      | Bucher | <b>-0.262 (0.006)</b> | -0.654 (0.006) | 0.130 (0.006)  | 0.108 (0.004) | 0.279 (0.006) | <b>0.753 (0.014)</b> | 1.009 (0.023) | 0.198 (0.004) |
| 107      | MAIC   | -0.001 (0.005)        | -0.317 (0.005) | 0.314 (0.005)  | 0.025 (0.001) | 0.127 (0.005) | 0.953 (0.007)        | 1.016 (0.023) | 0.159 (0.004) |
| 107      | STC    | <b>0.124 (0.006)</b>  | -0.229 (0.006) | 0.478 (0.006)  | 0.050 (0.002) | 0.179 (0.006) | <b>0.887 (0.010)</b> | 0.971 (0.022) | 0.186 (0.004) |
| 107      | Bucher | <b>-0.263 (0.005)</b> | -0.563 (0.005) | 0.037 (0.005)  | 0.091 (0.003) | 0.268 (0.005) | <b>0.613 (0.015)</b> | 1.034 (0.023) | 0.148 (0.003) |
| 108      | MAIC   | 0.009 (0.004)         | -0.245 (0.004) | 0.262 (0.004)  | 0.016 (0.001) | 0.100 (0.004) | 0.953 (0.007)        | 1.031 (0.023) | 0.126 (0.003) |
| 108      | STC    | <b>0.124 (0.004)</b>  | -0.149 (0.004) | 0.397 (0.004)  | 0.034 (0.001) | 0.149 (0.004) | <b>0.860 (0.011)</b> | 1.016 (0.023) | 0.137 (0.003) |
| 108      | Bucher | <b>-0.251 (0.004)</b> | -0.493 (0.004) | -0.008 (0.004) | 0.077 (0.002) | 0.252 (0.004) | <b>0.482 (0.016)</b> | 1.034 (0.023) | 0.120 (0.003) |
| 109      | MAIC   | -0.040 (0.014)        | -0.751 (0.015) | 0.672 (0.014)  | 0.189 (0.009) | 0.344 (0.014) | <b>0.895 (0.010)</b> | 0.839 (0.020) | 0.433 (0.010) |
| 109      | STC    | -0.068 (0.012)        | -0.758 (0.012) | 0.621 (0.012)  | 0.144 (0.007) | 0.300 (0.012) | <b>0.933 (0.008)</b> | 0.940 (0.021) | 0.374 (0.008) |
| 109      | Bucher | <b>-0.265 (0.007)</b> | -0.695 (0.007) | 0.164 (0.007)  | 0.118 (0.004) | 0.285 (0.007) | <b>0.788 (0.013)</b> | 1.008 (0.023) | 0.217 (0.005) |
| 110      | MAIC   | -0.011 (0.010)        | -0.552 (0.010) | 0.531 (0.010)  | 0.095 (0.004) | 0.248 (0.010) | <b>0.916 (0.009)</b> | 0.899 (0.021) | 0.307 (0.007) |
| 110      | STC    | -0.034 (0.008)        | -0.525 (0.008) | 0.456 (0.008)  | 0.066 (0.003) | 0.208 (0.008) | 0.954 (0.007)        | 0.981 (0.022) | 0.255 (0.006) |
| 110      | Bucher | <b>-0.262 (0.005)</b> | -0.589 (0.005) | 0.065 (0.005)  | 0.095 (0.003) | 0.269 (0.005) | <b>0.657 (0.015)</b> | 1.025 (0.023) | 0.163 (0.004) |
| 111      | MAIC   | 0.000 (0.007)         | -0.415 (0.007) | 0.414 (0.007)  | 0.050 (0.002) | 0.181 (0.007) | 0.937 (0.008)        | 0.946 (0.021) | 0.224 (0.005) |
| 111      | STC    | -0.027 (0.006)        | -0.391 (0.006) | 0.336 (0.006)  | 0.035 (0.002) | 0.149 (0.006) | 0.938 (0.008)        | 0.999 (0.022) | 0.186 (0.004) |
| 111      | Bucher | <b>-0.254 (0.004)</b> | -0.516 (0.004) | 0.009 (0.004)  | 0.083 (0.002) | 0.257 (0.004) | <b>0.533 (0.016)</b> | 0.992 (0.022) | 0.135 (0.003) |
| 112      | MAIC   | -0.019 (0.012)        | -0.682 (0.013) | 0.645 (0.013)  | 0.152 (0.007) | 0.310 (0.012) | <b>0.910 (0.009)</b> | 0.870 (0.020) | 0.389 (0.009) |
| 112      | STC    | -0.084 (0.011)        | -0.764 (0.012) | 0.596 (0.011)  | 0.134 (0.006) | 0.294 (0.011) | 0.953 (0.007)        | 0.974 (0.022) | 0.356 (0.008) |
| 112      | Bucher | <b>-0.236 (0.007)</b> | -0.656 (0.007) | 0.183 (0.007)  | 0.102 (0.004) | 0.265 (0.007) | <b>0.802 (0.013)</b> | 0.991 (0.022) | 0.216 (0.005) |
| 113      | MAIC   | -0.010 (0.009)        | -0.516 (0.009) | 0.496 (0.009)  | 0.077 (0.003) | 0.223 (0.009) | <b>0.921 (0.009)</b> | 0.928 (0.021) | 0.278 (0.006) |
| 113      | STC    | -0.089 (0.008)        | -0.571 (0.008) | 0.392 (0.008)  | 0.067 (0.003) | 0.205 (0.008) | <b>0.934 (0.008)</b> | 1.012 (0.023) | 0.243 (0.005) |
| 113      | Bucher | <b>-0.231 (0.005)</b> | -0.550 (0.005) | 0.089 (0.005)  | 0.079 (0.003) | 0.240 (0.005) | <b>0.723 (0.014)</b> | 1.017 (0.023) | 0.160 (0.004) |
| 114      | MAIC   | -0.005 (0.007)        | -0.398 (0.007) | 0.387 (0.007)  | 0.044 (0.002) | 0.166 (0.007) | <b>0.923 (0.008)</b> | 0.955 (0.022) | 0.209 (0.005) |
| 114      | STC    | -0.084 (0.006)        | -0.441 (0.006) | 0.273 (0.006)  | 0.041 (0.002) | 0.162 (0.006) | <b>0.922 (0.008)</b> | 0.984 (0.022) | 0.185 (0.004) |
| 114      | Bucher | <b>-0.237 (0.004)</b> | -0.493 (0.004) | 0.020 (0.004)  | 0.073 (0.002) | 0.240 (0.004) | <b>0.542 (0.016)</b> | 1.009 (0.023) | 0.130 (0.003) |
| 115      | MAIC   | -0.012 (0.012)        | -0.633 (0.012) | 0.609 (0.013)  | 0.139 (0.007) | 0.296 (0.012) | <b>0.906 (0.009)</b> | 0.849 (0.020) | 0.373 (0.008) |
| 115      | STC    | <b>-0.183 (0.011)</b> | -0.852 (0.012) | 0.486 (0.011)  | 0.159 (0.007) | 0.319 (0.011) | <b>0.924 (0.008)</b> | 0.962 (0.022) | 0.355 (0.008) |
| 115      | Bucher | <b>-0.209 (0.007)</b> | -0.617 (0.007) | 0.200 (0.006)  | 0.088 (0.003) | 0.244 (0.007) | <b>0.840 (0.012)</b> | 0.990 (0.022) | 0.211 (0.005) |
| 116      | MAIC   | 0.004 (0.008)         | -0.474 (0.008) | 0.482 (0.009)  | 0.068 (0.003) | 0.212 (0.008) | <b>0.928 (0.008)</b> | 0.936 (0.021) | 0.261 (0.006) |
| 116      | STC    | <b>-0.156 (0.008)</b> | -0.630 (0.008) | 0.317 (0.008)  | 0.087 (0.004) | 0.240 (0.008) | <b>0.899 (0.010)</b> | 0.969 (0.022) | 0.249 (0.006) |
| 116      | Bucher | <b>-0.195 (0.005)</b> | -0.506 (0.005) | 0.116 (0.005)  | 0.061 (0.002) | 0.207 (0.005) | <b>0.785 (0.013)</b> | 1.047 (0.023) | 0.152 (0.003) |
| 117      | MAIC   | 0.002 (0.006)         | -0.371 (0.006) | 0.376 (0.007)  | 0.040 (0.002) | 0.162 (0.006) | 0.943 (0.007)        | 0.957 (0.022) | 0.199 (0.004) |
| 117      | STC    | <b>-0.166 (0.006)</b> | -0.518 (0.006) | 0.186 (0.006)  | 0.061 (0.002) | 0.202 (0.006) | <b>0.843 (0.012)</b> | 0.974 (0.022) | 0.184 (0.004) |
| 117      | Bucher | <b>-0.203 (0.004)</b> | -0.453 (0.004) | 0.047 (0.004)  | 0.057 (0.002) | 0.209 (0.004) | <b>0.634 (0.015)</b> | 1.007 (0.023) | 0.127 (0.003) |

Table 3: Performance metrics for each method and simulation scenario. Monte Carlo standard errors for each measure are presented in parentheses. ATE: average estimated marginal treatment effect for  $A$  vs.  $B$  (is equal to the bias as the true effect is zero); LCI: average lower bound of the 95 percent confidence interval; UCI: average upper bound of the 95 percent confidence interval; MSE: mean square error; MAE: mean absolute error; Cov: coverage rate of the 95 percent confidence intervals; VR: variability ratio; ESE: empirical standard error; MAIC: matching-adjusted indirect comparison; STC: simulated treatment comparison. (*continued*)

| Scenario | Method | ATE                   | LCI            | UCI            | MSE           | MAE           | Cov                  | VR            | ESE           |
|----------|--------|-----------------------|----------------|----------------|---------------|---------------|----------------------|---------------|---------------|
| 118      | MAIC   | -0.009 (0.012)        | -0.681 (0.013) | 0.663 (0.013)  | 0.147 (0.007) | 0.306 (0.012) | <b>0.916 (0.009)</b> | 0.893 (0.021) | 0.384 (0.009) |
| 118      | STC    | 0.000 (0.011)         | -0.679 (0.011) | 0.679 (0.011)  | 0.124 (0.006) | 0.282 (0.011) | 0.950 (0.007)        | 0.985 (0.022) | 0.352 (0.008) |
| 118      | Bucher | <b>-0.410 (0.007)</b> | -0.833 (0.007) | 0.014 (0.006)  | 0.213 (0.006) | 0.412 (0.007) | <b>0.532 (0.016)</b> | 1.014 (0.023) | 0.213 (0.005) |
| 119      | MAIC   | -0.006 (0.009)        | -0.518 (0.009) | 0.506 (0.010)  | 0.082 (0.004) | 0.231 (0.009) | <b>0.924 (0.008)</b> | 0.913 (0.021) | 0.286 (0.006) |
| 119      | STC    | 0.008 (0.008)         | -0.472 (0.008) | 0.489 (0.008)  | 0.063 (0.003) | 0.201 (0.008) | 0.949 (0.007)        | 0.976 (0.022) | 0.251 (0.006) |
| 119      | Bucher | <b>-0.416 (0.005)</b> | -0.739 (0.005) | -0.094 (0.005) | 0.201 (0.005) | 0.417 (0.005) | <b>0.299 (0.014)</b> | 0.990 (0.022) | 0.166 (0.004) |
| 120      | MAIC   | -0.008 (0.007)        | -0.406 (0.007) | 0.390 (0.007)  | 0.044 (0.002) | 0.165 (0.007) | <b>0.936 (0.008)</b> | 0.965 (0.022) | 0.211 (0.005) |
| 120      | STC    | 0.004 (0.006)         | -0.354 (0.006) | 0.361 (0.006)  | 0.033 (0.002) | 0.144 (0.006) | 0.945 (0.007)        | 0.999 (0.022) | 0.183 (0.004) |
| 120      | Bucher | <b>-0.427 (0.004)</b> | -0.686 (0.004) | -0.168 (0.004) | 0.200 (0.004) | 0.427 (0.004) | <b>0.091 (0.009)</b> | 0.987 (0.022) | 0.134 (0.003) |
| 121      | MAIC   | -0.017 (0.012)        | -0.660 (0.013) | 0.626 (0.012)  | 0.142 (0.006) | 0.303 (0.012) | <b>0.904 (0.009)</b> | 0.870 (0.020) | 0.377 (0.008) |
| 121      | STC    | -0.049 (0.012)        | -0.722 (0.012) | 0.624 (0.012)  | 0.142 (0.007) | 0.299 (0.012) | <b>0.925 (0.008)</b> | 0.917 (0.021) | 0.374 (0.008) |
| 121      | Bucher | <b>-0.390 (0.007)</b> | -0.807 (0.007) | 0.026 (0.007)  | 0.199 (0.006) | 0.395 (0.007) | <b>0.541 (0.016)</b> | 0.983 (0.022) | 0.216 (0.005) |
| 122      | MAIC   | 0.007 (0.009)         | -0.481 (0.009) | 0.496 (0.009)  | 0.072 (0.003) | 0.214 (0.009) | <b>0.918 (0.009)</b> | 0.926 (0.021) | 0.269 (0.006) |
| 122      | STC    | -0.021 (0.008)        | -0.497 (0.008) | 0.454 (0.008)  | 0.060 (0.003) | 0.195 (0.008) | 0.944 (0.007)        | 0.993 (0.022) | 0.244 (0.005) |
| 122      | Bucher | <b>-0.374 (0.005)</b> | -0.690 (0.005) | -0.058 (0.005) | 0.166 (0.004) | 0.375 (0.005) | <b>0.363 (0.015)</b> | 1.003 (0.022) | 0.161 (0.004) |
| 123      | MAIC   | 0.008 (0.006)         | -0.375 (0.006) | 0.390 (0.007)  | 0.040 (0.002) | 0.161 (0.006) | 0.941 (0.007)        | 0.977 (0.022) | 0.200 (0.004) |
| 123      | STC    | -0.016 (0.006)        | -0.369 (0.006) | 0.337 (0.006)  | 0.032 (0.001) | 0.142 (0.006) | 0.955 (0.007)        | 1.015 (0.023) | 0.178 (0.004) |
| 123      | Bucher | <b>-0.386 (0.004)</b> | -0.640 (0.004) | -0.133 (0.004) | 0.167 (0.003) | 0.387 (0.004) | <b>0.151 (0.011)</b> | 0.981 (0.022) | 0.132 (0.003) |
| 124      | MAIC   | 0.000 (0.011)         | -0.604 (0.012) | 0.603 (0.012)  | 0.124 (0.006) | 0.281 (0.011) | <b>0.902 (0.009)</b> | 0.873 (0.020) | 0.353 (0.008) |
| 124      | STC    | -0.065 (0.011)        | -0.725 (0.011) | 0.595 (0.011)  | 0.119 (0.005) | 0.278 (0.011) | 0.948 (0.007)        | 0.992 (0.022) | 0.339 (0.008) |
| 124      | Bucher | <b>-0.324 (0.007)</b> | -0.731 (0.007) | 0.082 (0.006)  | 0.149 (0.005) | 0.335 (0.007) | <b>0.669 (0.015)</b> | 0.995 (0.022) | 0.209 (0.005) |
| 125      | MAIC   | -0.006 (0.008)        | -0.470 (0.008) | 0.457 (0.009)  | 0.065 (0.003) | 0.203 (0.008) | <b>0.931 (0.008)</b> | 0.930 (0.021) | 0.254 (0.006) |
| 125      | STC    | -0.069 (0.008)        | -0.538 (0.008) | 0.400 (0.008)  | 0.064 (0.003) | 0.201 (0.008) | <b>0.933 (0.008)</b> | 0.982 (0.022) | 0.244 (0.005) |
| 125      | Bucher | <b>-0.330 (0.005)</b> | -0.640 (0.005) | -0.020 (0.005) | 0.135 (0.004) | 0.332 (0.005) | <b>0.460 (0.016)</b> | 0.980 (0.022) | 0.161 (0.004) |
| 126      | MAIC   | 0.003 (0.006)         | -0.365 (0.006) | 0.370 (0.006)  | 0.037 (0.002) | 0.153 (0.006) | 0.942 (0.007)        | 0.979 (0.022) | 0.192 (0.004) |
| 126      | STC    | -0.066 (0.006)        | -0.414 (0.006) | 0.283 (0.006)  | 0.036 (0.002) | 0.152 (0.006) | <b>0.935 (0.008)</b> | 0.999 (0.022) | 0.178 (0.004) |
| 126      | Bucher | <b>-0.330 (0.004)</b> | -0.578 (0.004) | -0.081 (0.004) | 0.124 (0.003) | 0.330 (0.004) | <b>0.258 (0.014)</b> | 1.013 (0.023) | 0.125 (0.003) |
| 127      | MAIC   | 0.021 (0.012)         | -0.618 (0.012) | 0.661 (0.012)  | 0.135 (0.006) | 0.296 (0.012) | <b>0.899 (0.010)</b> | 0.890 (0.021) | 0.367 (0.008) |
| 127      | STC    | 0.109 (0.011)         | -0.560 (0.011) | 0.779 (0.011)  | 0.134 (0.006) | 0.294 (0.011) | <b>0.932 (0.008)</b> | 0.979 (0.022) | 0.349 (0.008) |
| 127      | Bucher | <b>-0.623 (0.007)</b> | -1.042 (0.007) | -0.204 (0.006) | 0.432 (0.009) | 0.623 (0.007) | <b>0.146 (0.011)</b> | 1.017 (0.023) | 0.210 (0.005) |
| 128      | MAIC   | 0.003 (0.008)         | -0.484 (0.008) | 0.491 (0.009)  | 0.071 (0.003) | 0.213 (0.008) | <b>0.921 (0.009)</b> | 0.934 (0.021) | 0.266 (0.006) |
| 128      | STC    | 0.102 (0.008)         | -0.374 (0.008) | 0.577 (0.008)  | 0.068 (0.003) | 0.208 (0.008) | <b>0.928 (0.008)</b> | 1.013 (0.023) | 0.239 (0.005) |
| 128      | Bucher | <b>-0.627 (0.005)</b> | -0.946 (0.005) | -0.308 (0.005) | 0.418 (0.006) | 0.627 (0.005) | <b>0.018 (0.004)</b> | 1.031 (0.023) | 0.158 (0.004) |
| 129      | MAIC   | 0.003 (0.006)         | -0.376 (0.006) | 0.383 (0.006)  | 0.038 (0.002) | 0.153 (0.006) | 0.948 (0.007)        | 0.997 (0.023) | 0.194 (0.004) |
| 129      | STC    | <b>0.100 (0.006)</b>  | -0.252 (0.006) | 0.453 (0.006)  | 0.041 (0.002) | 0.160 (0.006) | <b>0.918 (0.009)</b> | 1.029 (0.023) | 0.175 (0.004) |
| 129      | Bucher | <b>-0.616 (0.004)</b> | -0.871 (0.004) | -0.361 (0.004) | 0.396 (0.005) | 0.616 (0.004) | <b>0.002 (0.001)</b> | 1.014 (0.023) | 0.128 (0.003) |
| 130      | MAIC   | 0.018 (0.011)         | -0.603 (0.012) | 0.640 (0.012)  | 0.131 (0.006) | 0.287 (0.011) | <b>0.904 (0.009)</b> | 0.878 (0.020) | 0.361 (0.008) |
| 130      | STC    | 0.138 (0.011)         | -0.526 (0.011) | 0.803 (0.011)  | 0.145 (0.007) | 0.301 (0.011) | <b>0.920 (0.009)</b> | 0.954 (0.021) | 0.355 (0.008) |
| 130      | Bucher | <b>-0.560 (0.007)</b> | -0.973 (0.007) | -0.146 (0.007) | 0.359 (0.008) | 0.560 (0.007) | <b>0.245 (0.014)</b> | 0.985 (0.022) | 0.214 (0.005) |
| 131      | MAIC   | 0.017 (0.008)         | -0.452 (0.008) | 0.487 (0.009)  | 0.069 (0.003) | 0.210 (0.008) | <b>0.921 (0.009)</b> | 0.914 (0.021) | 0.262 (0.006) |
| 131      | STC    | 0.116 (0.008)         | -0.354 (0.008) | 0.586 (0.008)  | 0.075 (0.004) | 0.217 (0.008) | <b>0.915 (0.009)</b> | 0.964 (0.022) | 0.249 (0.006) |
| 131      | Bucher | <b>-0.556 (0.005)</b> | -0.870 (0.005) | -0.242 (0.005) | 0.335 (0.006) | 0.556 (0.005) | <b>0.057 (0.007)</b> | 1.002 (0.022) | 0.160 (0.004) |
| 132      | MAIC   | 0.017 (0.006)         | -0.349 (0.006) | 0.383 (0.006)  | 0.039 (0.002) | 0.162 (0.006) | 0.937 (0.008)        | 0.943 (0.021) | 0.198 (0.004) |
| 132      | STC    | <b>0.118 (0.006)</b>  | -0.230 (0.006) | 0.466 (0.006)  | 0.048 (0.002) | 0.178 (0.006) | <b>0.883 (0.010)</b> | 0.954 (0.021) | 0.186 (0.004) |
| 132      | Bucher | <b>-0.557 (0.004)</b> | -0.808 (0.004) | -0.306 (0.004) | 0.327 (0.005) | 0.557 (0.004) | <b>0.006 (0.002)</b> | 0.995 (0.022) | 0.129 (0.003) |
| 133      | MAIC   | 0.016 (0.011)         | -0.572 (0.011) | 0.604 (0.011)  | 0.118 (0.005) | 0.277 (0.011) | <b>0.897 (0.010)</b> | 0.874 (0.020) | 0.343 (0.008) |
| 133      | STC    | 0.116 (0.011)         | -0.541 (0.011) | 0.772 (0.011)  | 0.131 (0.006) | 0.289 (0.011) | <b>0.936 (0.008)</b> | 0.977 (0.022) | 0.343 (0.008) |
| 133      | Bucher | <b>-0.477 (0.007)</b> | -0.883 (0.007) | -0.072 (0.007) | 0.274 (0.007) | 0.479 (0.007) | <b>0.375 (0.015)</b> | 0.965 (0.022) | 0.214 (0.005) |
| 134      | MAIC   | 0.026 (0.008)         | -0.432 (0.008) | 0.484 (0.008)  | 0.061 (0.003) | 0.199 (0.008) | <b>0.929 (0.008)</b> | 0.954 (0.022) | 0.245 (0.005) |
| 134      | STC    | 0.109 (0.008)         | -0.357 (0.008) | 0.574 (0.008)  | 0.071 (0.003) | 0.213 (0.008) | <b>0.912 (0.009)</b> | 0.976 (0.022) | 0.243 (0.005) |
| 134      | Bucher | <b>-0.475 (0.005)</b> | -0.784 (0.005) | -0.167 (0.005) | 0.250 (0.005) | 0.476 (0.005) | <b>0.139 (0.011)</b> | 1.013 (0.023) | 0.155 (0.003) |
| 135      | MAIC   | 0.025 (0.006)         | -0.333 (0.006) | 0.382 (0.006)  | 0.034 (0.002) | 0.146 (0.006) | 0.946 (0.007)        | 1.003 (0.023) | 0.182 (0.004) |
| 135      | STC    | <b>0.112 (0.005)</b>  | -0.232 (0.005) | 0.457 (0.005)  | 0.041 (0.002) | 0.161 (0.005) | <b>0.910 (0.009)</b> | 1.041 (0.023) | 0.169 (0.004) |
| 135      | Bucher | <b>-0.478 (0.004)</b> | -0.725 (0.004) | -0.231 (0.004) | 0.244 (0.004) | 0.478 (0.004) | <b>0.031 (0.005)</b> | 1.022 (0.023) | 0.123 (0.003) |
| 136      | MAIC   | -0.013 (0.010)        | -0.603 (0.011) | 0.577 (0.011)  | 0.108 (0.005) | 0.261 (0.010) | <b>0.917 (0.009)</b> | 0.916 (0.021) | 0.329 (0.007) |
| 136      | STC    | -0.084 (0.011)        | -0.708 (0.011) | 0.540 (0.011)  | 0.122 (0.006) | 0.277 (0.011) | <b>0.931 (0.008)</b> | 0.936 (0.021) | 0.340 (0.008) |
| 136      | Bucher | <b>-0.244 (0.007)</b> | -0.671 (0.007) | 0.183 (0.007)  | 0.109 (0.004) | 0.276 (0.007) | <b>0.815 (0.012)</b> | 0.984 (0.022) | 0.222 (0.005) |
| 137      | MAIC   | -0.018 (0.007)        | -0.467 (0.008) | 0.431 (0.008)  | 0.056 (0.003) | 0.187 (0.007) | <b>0.933 (0.008)</b> | 0.971 (0.022) | 0.236 (0.005) |
| 137      | STC    | -0.077 (0.007)        | -0.524 (0.007) | 0.369 (0.007)  | 0.059 (0.003) | 0.190 (0.007) | <b>0.934 (0.008)</b> | 0.992 (0.022) | 0.230 (0.005) |
| 137      | Bucher | <b>-0.244 (0.005)</b> | -0.569 (0.005) | 0.082 (0.005)  | 0.087 (0.003) | 0.253 (0.005) | <b>0.703 (0.014)</b> | 0.998 (0.022) | 0.166 (0.004) |

Table 3: Performance metrics for each method and simulation scenario. Monte Carlo standard errors for each measure are presented in parentheses. ATE: average estimated marginal treatment effect for  $A$  vs.  $B$  (is equal to the bias as the true effect is zero); LCI: average lower bound of the 95 percent confidence interval; UCI: average upper bound of the 95 percent confidence interval; MSE: mean square error; MAE: mean absolute error; Cov: coverage rate of the 95 percent confidence intervals; VR: variability ratio; ESE: empirical standard error; MAIC: matching-adjusted indirect comparison; STC: simulated treatment comparison. (*continued*)

| Scenario | Method | ATE                   | LCI            | UCI            | MSE           | MAE           | Cov                  | VR            | ESE           |
|----------|--------|-----------------------|----------------|----------------|---------------|---------------|----------------------|---------------|---------------|
| 138      | MAIC   | 0.011 (0.006)         | -0.337 (0.006) | 0.359 (0.006)  | 0.033 (0.001) | 0.145 (0.006) | 0.941 (0.007)        | 0.981 (0.022) | 0.181 (0.004) |
| 138      | STC    | -0.049 (0.005)        | -0.386 (0.005) | 0.288 (0.005)  | 0.032 (0.001) | 0.141 (0.005) | <b>0.933 (0.008)</b> | 1.005 (0.023) | 0.171 (0.004) |
| 138      | Bucher | <b>-0.230 (0.004)</b> | -0.492 (0.004) | 0.032 (0.004)  | 0.070 (0.002) | 0.235 (0.004) | <b>0.613 (0.015)</b> | 1.019 (0.023) | 0.131 (0.003) |
| 139      | MAIC   | -0.012 (0.010)        | -0.558 (0.010) | 0.534 (0.010)  | 0.094 (0.004) | 0.245 (0.010) | <b>0.921 (0.009)</b> | 0.909 (0.021) | 0.306 (0.007) |
| 139      | STC    | -0.152 (0.010)        | -0.766 (0.010) | 0.461 (0.010)  | 0.120 (0.005) | 0.277 (0.010) | <b>0.928 (0.008)</b> | 1.008 (0.023) | 0.311 (0.007) |
| 139      | Bucher | <b>-0.216 (0.006)</b> | -0.633 (0.007) | 0.201 (0.006)  | 0.089 (0.003) | 0.245 (0.006) | <b>0.849 (0.011)</b> | 1.038 (0.023) | 0.205 (0.005) |
| 140      | MAIC   | -0.009 (0.007)        | -0.428 (0.007) | 0.410 (0.007)  | 0.051 (0.002) | 0.180 (0.007) | <b>0.934 (0.008)</b> | 0.949 (0.021) | 0.225 (0.005) |
| 140      | STC    | <b>-0.137 (0.007)</b> | -0.577 (0.007) | 0.303 (0.007)  | 0.068 (0.003) | 0.207 (0.007) | <b>0.915 (0.009)</b> | 1.016 (0.023) | 0.221 (0.005) |
| 140      | Bucher | <b>-0.215 (0.005)</b> | -0.533 (0.005) | 0.103 (0.005)  | 0.071 (0.002) | 0.228 (0.005) | <b>0.758 (0.014)</b> | 1.025 (0.023) | 0.158 (0.004) |
| 141      | MAIC   | -0.009 (0.005)        | -0.339 (0.005) | 0.320 (0.005)  | 0.027 (0.001) | 0.130 (0.005) | 0.949 (0.007)        | 1.032 (0.023) | 0.163 (0.004) |
| 141      | STC    | <b>-0.140 (0.005)</b> | -0.470 (0.005) | 0.190 (0.005)  | 0.047 (0.002) | 0.177 (0.005) | <b>0.873 (0.011)</b> | 1.017 (0.023) | 0.165 (0.004) |
| 141      | Bucher | <b>-0.211 (0.004)</b> | -0.466 (0.004) | 0.044 (0.004)  | 0.061 (0.002) | 0.216 (0.004) | <b>0.640 (0.015)</b> | 1.020 (0.023) | 0.128 (0.003) |
| 142      | MAIC   | -0.022 (0.009)        | -0.541 (0.009) | 0.497 (0.010)  | 0.081 (0.004) | 0.228 (0.009) | <b>0.922 (0.008)</b> | 0.929 (0.021) | 0.285 (0.006) |
| 142      | STC    | <b>-0.268 (0.010)</b> | -0.877 (0.010) | 0.341 (0.010)  | 0.172 (0.007) | 0.335 (0.010) | <b>0.860 (0.011)</b> | 0.981 (0.022) | 0.317 (0.007) |
| 142      | Bucher | <b>-0.175 (0.006)</b> | -0.584 (0.006) | 0.235 (0.006)  | 0.070 (0.003) | 0.213 (0.006) | <b>0.890 (0.010)</b> | 1.052 (0.024) | 0.198 (0.004) |
| 143      | MAIC   | -0.013 (0.007)        | -0.416 (0.007) | 0.389 (0.007)  | 0.049 (0.002) | 0.177 (0.007) | <b>0.912 (0.009)</b> | 0.929 (0.021) | 0.221 (0.005) |
| 143      | STC    | <b>-0.245 (0.007)</b> | -0.680 (0.007) | 0.190 (0.007)  | 0.113 (0.004) | 0.280 (0.007) | <b>0.796 (0.013)</b> | 0.967 (0.022) | 0.229 (0.005) |
| 143      | Bucher | <b>-0.175 (0.005)</b> | -0.486 (0.005) | 0.137 (0.005)  | 0.056 (0.002) | 0.196 (0.005) | <b>0.803 (0.013)</b> | 0.997 (0.022) | 0.159 (0.004) |
| 144      | MAIC   | 0.001 (0.005)         | -0.318 (0.005) | 0.320 (0.005)  | 0.027 (0.001) | 0.133 (0.005) | 0.944 (0.007)        | 0.984 (0.022) | 0.165 (0.004) |
| 144      | STC    | <b>-0.236 (0.005)</b> | -0.562 (0.005) | 0.089 (0.005)  | 0.084 (0.003) | 0.249 (0.005) | <b>0.676 (0.015)</b> | 0.983 (0.022) | 0.169 (0.004) |
| 144      | Bucher | <b>-0.177 (0.004)</b> | -0.427 (0.004) | 0.073 (0.004)  | 0.048 (0.002) | 0.187 (0.004) | <b>0.714 (0.014)</b> | 0.992 (0.022) | 0.129 (0.003) |
| 145      | MAIC   | 0.017 (0.010)         | -0.549 (0.010) | 0.583 (0.010)  | 0.101 (0.005) | 0.253 (0.010) | <b>0.911 (0.009)</b> | 0.910 (0.021) | 0.317 (0.007) |
| 145      | STC    | 0.011 (0.010)         | -0.605 (0.011) | 0.627 (0.010)  | 0.108 (0.005) | 0.262 (0.010) | 0.937 (0.008)        | 0.955 (0.021) | 0.329 (0.007) |
| 145      | Bucher | <b>-0.380 (0.007)</b> | -0.803 (0.007) | 0.044 (0.007)  | 0.192 (0.006) | 0.384 (0.007) | <b>0.585 (0.016)</b> | 0.986 (0.022) | 0.219 (0.005) |
| 146      | MAIC   | -0.008 (0.007)        | -0.439 (0.007) | 0.423 (0.007)  | 0.052 (0.002) | 0.181 (0.007) | 0.937 (0.008)        | 0.960 (0.022) | 0.229 (0.005) |
| 146      | STC    | -0.003 (0.007)        | -0.443 (0.007) | 0.437 (0.007)  | 0.053 (0.002) | 0.183 (0.007) | 0.947 (0.007)        | 0.978 (0.022) | 0.229 (0.005) |
| 146      | Bucher | <b>-0.385 (0.005)</b> | -0.707 (0.005) | -0.062 (0.005) | 0.174 (0.004) | 0.385 (0.005) | <b>0.347 (0.015)</b> | 1.013 (0.023) | 0.162 (0.004) |
| 147      | MAIC   | 0.001 (0.005)         | -0.336 (0.005) | 0.338 (0.006)  | 0.030 (0.001) | 0.139 (0.005) | 0.940 (0.008)        | 0.993 (0.022) | 0.173 (0.004) |
| 147      | STC    | -0.003 (0.005)        | -0.333 (0.005) | 0.328 (0.005)  | 0.027 (0.001) | 0.132 (0.005) | 0.958 (0.006)        | 1.023 (0.023) | 0.165 (0.004) |
| 147      | Bucher | <b>-0.392 (0.004)</b> | -0.651 (0.004) | -0.133 (0.004) | 0.170 (0.003) | 0.392 (0.004) | <b>0.141 (0.011)</b> | 1.028 (0.023) | 0.129 (0.003) |
| 148      | MAIC   | 0.001 (0.010)         | -0.534 (0.010) | 0.536 (0.010)  | 0.091 (0.004) | 0.238 (0.010) | <b>0.909 (0.009)</b> | 0.906 (0.021) | 0.301 (0.007) |
| 148      | STC    | -0.057 (0.010)        | -0.664 (0.011) | 0.550 (0.010)  | 0.108 (0.005) | 0.260 (0.010) | <b>0.936 (0.008)</b> | 0.957 (0.022) | 0.323 (0.007) |
| 148      | Bucher | <b>-0.332 (0.007)</b> | -0.748 (0.007) | 0.084 (0.007)  | 0.159 (0.005) | 0.342 (0.007) | <b>0.644 (0.015)</b> | 0.962 (0.022) | 0.221 (0.005) |
| 149      | MAIC   | -0.003 (0.007)        | -0.417 (0.007) | 0.410 (0.007)  | 0.049 (0.002) | 0.178 (0.007) | <b>0.930 (0.008)</b> | 0.952 (0.022) | 0.222 (0.005) |
| 149      | STC    | -0.046 (0.007)        | -0.481 (0.007) | 0.389 (0.007)  | 0.054 (0.002) | 0.183 (0.007) | <b>0.934 (0.008)</b> | 0.977 (0.022) | 0.227 (0.005) |
| 149      | Bucher | <b>-0.337 (0.005)</b> | -0.653 (0.005) | -0.021 (0.005) | 0.139 (0.004) | 0.338 (0.005) | <b>0.441 (0.016)</b> | 1.009 (0.023) | 0.160 (0.004) |
| 150      | MAIC   | 0.002 (0.005)         | -0.324 (0.005) | 0.327 (0.006)  | 0.029 (0.001) | 0.135 (0.005) | <b>0.933 (0.008)</b> | 0.975 (0.022) | 0.170 (0.004) |
| 150      | STC    | -0.043 (0.005)        | -0.369 (0.005) | 0.283 (0.005)  | 0.031 (0.001) | 0.137 (0.005) | <b>0.933 (0.008)</b> | 0.980 (0.022) | 0.170 (0.004) |
| 150      | Bucher | <b>-0.331 (0.004)</b> | -0.584 (0.004) | -0.077 (0.004) | 0.126 (0.003) | 0.331 (0.004) | <b>0.264 (0.014)</b> | 0.999 (0.022) | 0.130 (0.003) |
| 151      | MAIC   | -0.004 (0.009)        | -0.520 (0.009) | 0.512 (0.010)  | 0.087 (0.004) | 0.236 (0.009) | <b>0.893 (0.010)</b> | 0.893 (0.020) | 0.295 (0.007) |
| 151      | STC    | -0.105 (0.010)        | -0.709 (0.010) | 0.500 (0.010)  | 0.114 (0.005) | 0.267 (0.010) | <b>0.916 (0.009)</b> | 0.961 (0.022) | 0.321 (0.007) |
| 151      | Bucher | <b>-0.266 (0.007)</b> | -0.674 (0.007) | 0.143 (0.006)  | 0.113 (0.004) | 0.283 (0.007) | <b>0.759 (0.014)</b> | 1.007 (0.023) | 0.207 (0.005) |
| 152      | MAIC   | -0.010 (0.007)        | -0.413 (0.007) | 0.393 (0.007)  | 0.043 (0.002) | 0.168 (0.007) | 0.941 (0.007)        | 0.989 (0.022) | 0.208 (0.005) |
| 152      | STC    | -0.105 (0.007)        | -0.536 (0.007) | 0.326 (0.007)  | 0.059 (0.002) | 0.195 (0.007) | <b>0.931 (0.008)</b> | 1.004 (0.023) | 0.219 (0.005) |
| 152      | Bucher | <b>-0.278 (0.005)</b> | -0.589 (0.005) | 0.033 (0.005)  | 0.101 (0.003) | 0.280 (0.005) | <b>0.599 (0.015)</b> | 1.017 (0.023) | 0.156 (0.003) |
| 153      | MAIC   | 0.007 (0.005)         | -0.310 (0.005) | 0.323 (0.006)  | 0.029 (0.001) | 0.136 (0.005) | <b>0.926 (0.008)</b> | 0.955 (0.021) | 0.169 (0.004) |
| 153      | STC    | <b>-0.095 (0.005)</b> | -0.417 (0.005) | 0.228 (0.005)  | 0.037 (0.002) | 0.152 (0.005) | <b>0.900 (0.009)</b> | 0.986 (0.022) | 0.167 (0.004) |
| 153      | Bucher | <b>-0.265 (0.004)</b> | -0.515 (0.004) | -0.016 (0.004) | 0.086 (0.002) | 0.267 (0.004) | <b>0.458 (0.016)</b> | 1.017 (0.023) | 0.125 (0.003) |
| 154      | MAIC   | 0.018 (0.010)         | -0.530 (0.010) | 0.566 (0.010)  | 0.093 (0.005) | 0.239 (0.010) | <b>0.921 (0.009)</b> | 0.916 (0.021) | 0.305 (0.007) |
| 154      | STC    | 0.136 (0.010)         | -0.471 (0.010) | 0.742 (0.011)  | 0.125 (0.006) | 0.278 (0.010) | <b>0.912 (0.009)</b> | 0.949 (0.021) | 0.326 (0.007) |
| 154      | Bucher | <b>-0.565 (0.007)</b> | -0.986 (0.007) | -0.145 (0.006) | 0.365 (0.008) | 0.566 (0.007) | <b>0.226 (0.013)</b> | 1.009 (0.023) | 0.213 (0.005) |
| 155      | MAIC   | 0.005 (0.007)         | -0.414 (0.007) | 0.424 (0.007)  | 0.045 (0.002) | 0.170 (0.007) | 0.943 (0.007)        | 1.005 (0.023) | 0.213 (0.005) |
| 155      | STC    | <b>0.118 (0.007)</b>  | -0.316 (0.007) | 0.552 (0.007)  | 0.061 (0.003) | 0.198 (0.007) | <b>0.914 (0.009)</b> | 1.024 (0.023) | 0.216 (0.005) |
| 155      | Bucher | <b>-0.566 (0.005)</b> | -0.886 (0.005) | -0.247 (0.005) | 0.345 (0.006) | 0.566 (0.005) | <b>0.059 (0.007)</b> | 1.040 (0.023) | 0.157 (0.004) |
| 156      | MAIC   | 0.005 (0.005)         | -0.322 (0.005) | 0.331 (0.005)  | 0.028 (0.001) | 0.133 (0.005) | <b>0.936 (0.008)</b> | 0.999 (0.022) | 0.167 (0.004) |
| 156      | STC    | <b>0.131 (0.005)</b>  | -0.195 (0.005) | 0.457 (0.005)  | 0.046 (0.002) | 0.171 (0.005) | <b>0.866 (0.011)</b> | 0.987 (0.022) | 0.169 (0.004) |
| 156      | Bucher | <b>-0.562 (0.004)</b> | -0.818 (0.004) | -0.306 (0.004) | 0.333 (0.005) | 0.562 (0.004) | <b>0.014 (0.004)</b> | 0.997 (0.022) | 0.131 (0.003) |
| 157      | MAIC   | 0.011 (0.009)         | -0.509 (0.009) | 0.532 (0.009)  | 0.081 (0.004) | 0.228 (0.009) | <b>0.927 (0.008)</b> | 0.932 (0.021) | 0.285 (0.006) |
| 157      | STC    | 0.138 (0.010)         | -0.460 (0.010) | 0.736 (0.010)  | 0.121 (0.006) | 0.278 (0.010) | <b>0.923 (0.008)</b> | 0.957 (0.022) | 0.319 (0.007) |
| 157      | Bucher | <b>-0.477 (0.007)</b> | -0.890 (0.007) | -0.063 (0.006) | 0.272 (0.007) | 0.478 (0.007) | <b>0.396 (0.015)</b> | 0.998 (0.022) | 0.211 (0.005) |

Table 3: Performance metrics for each method and simulation scenario. Monte Carlo standard errors for each measure are presented in parentheses. ATE: average estimated marginal treatment effect for  $A$  vs.  $B$  (is equal to the bias as the true effect is zero); LCI: average lower bound of the 95 percent confidence interval; UCI: average upper bound of the 95 percent confidence interval; MSE: mean square error; MAE: mean absolute error; Cov: coverage rate of the 95 percent confidence intervals; VR: variability ratio; ESE: empirical standard error; MAIC: matching-adjusted indirect comparison; STC: simulated treatment comparison. (*continued*)

| Scenario | Method | ATE                   | LCI            | UCI            | MSE           | MAE           | Cov                  | VR            | ESE           |
|----------|--------|-----------------------|----------------|----------------|---------------|---------------|----------------------|---------------|---------------|
| 158      | MAIC   | 0.010 (0.007)         | -0.395 (0.007) | 0.415 (0.007)  | 0.050 (0.002) | 0.179 (0.007) | <b>0.917 (0.009)</b> | 0.929 (0.021) | 0.223 (0.005) |
| 158      | STC    | <b>0.126 (0.007)</b>  | -0.303 (0.007) | 0.556 (0.007)  | 0.065 (0.003) | 0.206 (0.007) | <b>0.908 (0.009)</b> | 0.987 (0.022) | 0.222 (0.005) |
| 158      | Bucher | <b>-0.471 (0.005)</b> | -0.786 (0.005) | -0.157 (0.005) | 0.249 (0.005) | 0.471 (0.005) | <b>0.153 (0.011)</b> | 0.985 (0.022) | 0.163 (0.004) |
| 159      | MAIC   | 0.009 (0.005)         | -0.310 (0.005) | 0.327 (0.005)  | 0.026 (0.001) | 0.132 (0.005) | 0.953 (0.007)        | 1.008 (0.023) | 0.161 (0.004) |
| 159      | STC    | <b>0.141 (0.005)</b>  | -0.182 (0.005) | 0.463 (0.005)  | 0.047 (0.002) | 0.176 (0.005) | <b>0.850 (0.011)</b> | 0.991 (0.022) | 0.166 (0.004) |
| 159      | Bucher | <b>-0.470 (0.004)</b> | -0.722 (0.004) | -0.218 (0.004) | 0.236 (0.004) | 0.470 (0.004) | <b>0.043 (0.006)</b> | 1.034 (0.023) | 0.124 (0.003) |
| 160      | MAIC   | 0.024 (0.009)         | -0.491 (0.009) | 0.538 (0.009)  | 0.080 (0.003) | 0.228 (0.009) | <b>0.913 (0.009)</b> | 0.931 (0.021) | 0.282 (0.006) |
| 160      | STC    | 0.124 (0.010)         | -0.479 (0.010) | 0.727 (0.010)  | 0.113 (0.005) | 0.268 (0.010) | <b>0.924 (0.008)</b> | 0.984 (0.022) | 0.313 (0.007) |
| 160      | Bucher | <b>-0.380 (0.007)</b> | -0.788 (0.007) | 0.028 (0.006)  | 0.188 (0.005) | 0.386 (0.007) | <b>0.550 (0.016)</b> | 1.001 (0.022) | 0.208 (0.005) |
| 161      | MAIC   | 0.001 (0.007)         | -0.398 (0.007) | 0.400 (0.007)  | 0.044 (0.002) | 0.169 (0.007) | <b>0.936 (0.008)</b> | 0.971 (0.022) | 0.210 (0.005) |
| 161      | STC    | <b>0.122 (0.007)</b>  | -0.307 (0.007) | 0.551 (0.007)  | 0.064 (0.003) | 0.200 (0.007) | <b>0.908 (0.009)</b> | 0.991 (0.022) | 0.221 (0.005) |
| 161      | Bucher | <b>-0.388 (0.005)</b> | -0.699 (0.005) | -0.077 (0.005) | 0.177 (0.004) | 0.389 (0.005) | <b>0.312 (0.015)</b> | 0.980 (0.022) | 0.162 (0.004) |
| 162      | MAIC   | 0.012 (0.005)         | -0.302 (0.005) | 0.325 (0.005)  | 0.023 (0.001) | 0.123 (0.005) | 0.952 (0.007)        | 1.047 (0.024) | 0.153 (0.003) |
| 162      | STC    | <b>0.122 (0.005)</b>  | -0.199 (0.005) | 0.442 (0.005)  | 0.038 (0.002) | 0.157 (0.005) | <b>0.901 (0.009)</b> | 1.075 (0.024) | 0.152 (0.003) |
| 162      | Bucher | <b>-0.379 (0.004)</b> | -0.628 (0.004) | -0.130 (0.004) | 0.159 (0.003) | 0.379 (0.004) | <b>0.147 (0.011)</b> | 1.020 (0.023) | 0.124 (0.003) |

## Appendix E: Nested loop plots of performance measures

Nested loop plots illustrating the bias, variability ratio, empirical coverage rate of 95% confidence intervals, empirical standard error, and mean square error, across all simulation scenarios are presented in the main text.

Figure 3 illustrates the MAE across all 162 simulation scenarios in a nested loop plot. Figure 4 displays the standardized biases, Figure 5 presents the average 95% confidence interval widths, Figure 6 shows the percentage of replicates with less accurate point estimates than the Bucher method for MAIC and STC. Figure 7 presents the average percentage reduction in effective sample size for MAIC. Figure 8 displays a plot of the bias converging over the simulations in Scenario 1 for each method.



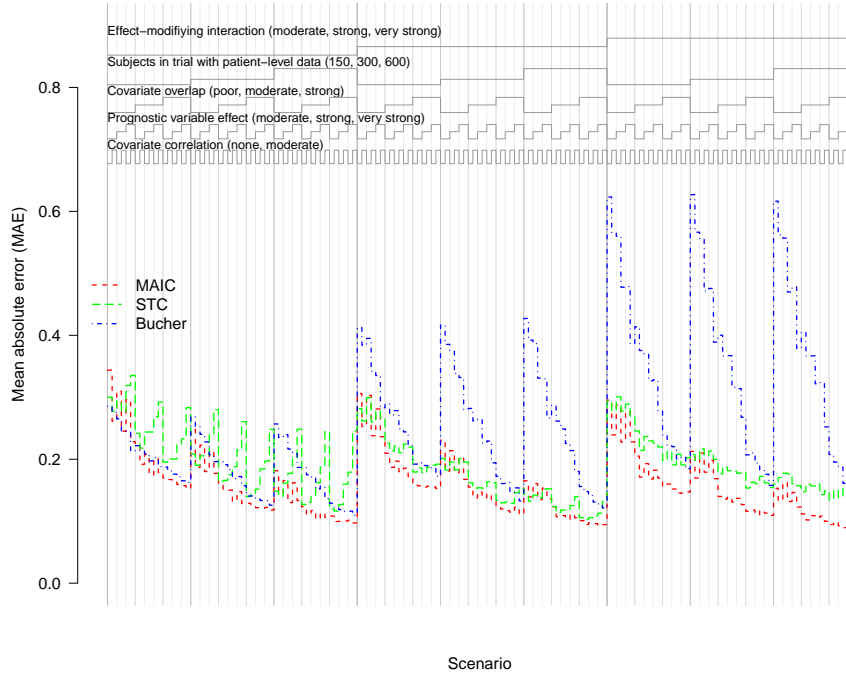

Figure 3: Mean absolute error (MAE) across all scenarios. MAIC: matching-adjusted indirect comparison; STC: simulated treatment comparison.

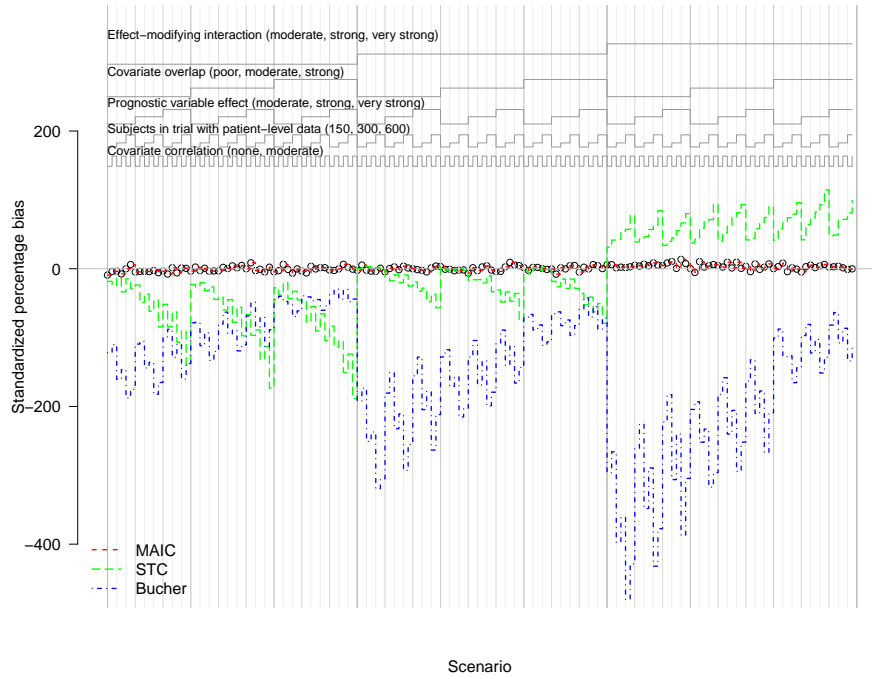

Figure 4: Standardized bias across all simulation scenarios. MAIC: matching-adjusted indirect comparison; STC: simulated treatment comparison.



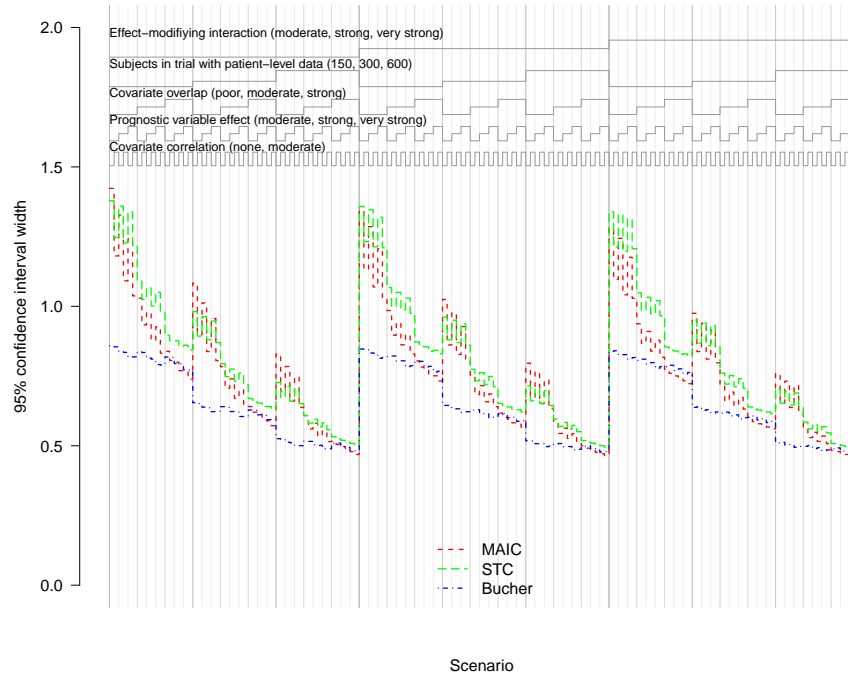

Figure 5: Average 95% confidence interval width across all scenarios. MAIC: matching-adjusted indirect comparison; STC: simulated treatment comparison.

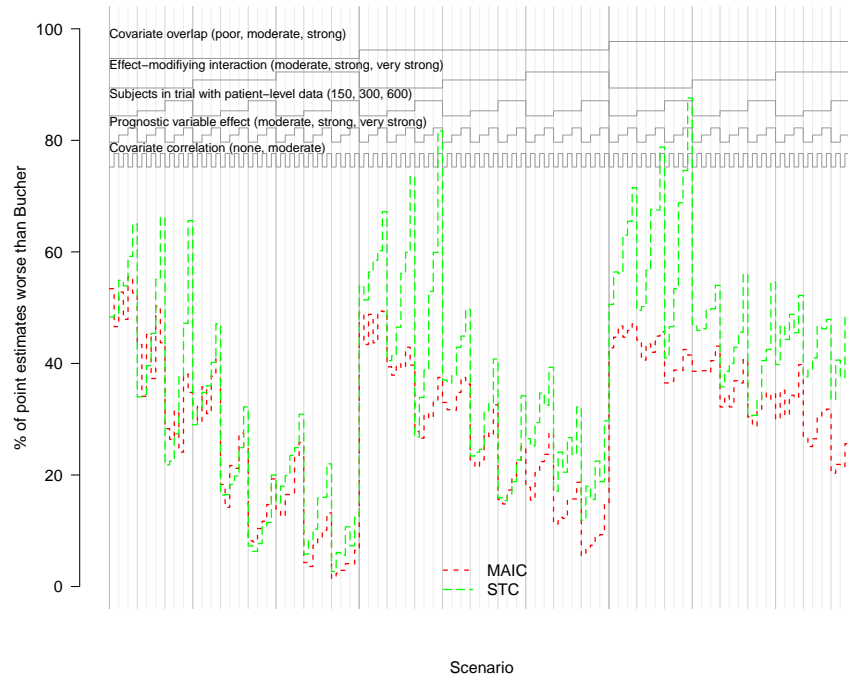

Figure 6: Percentage of replicates less accurate than Bucher. MAIC: matching-adjusted indirect comparison; STC: simulated treatment comparison.

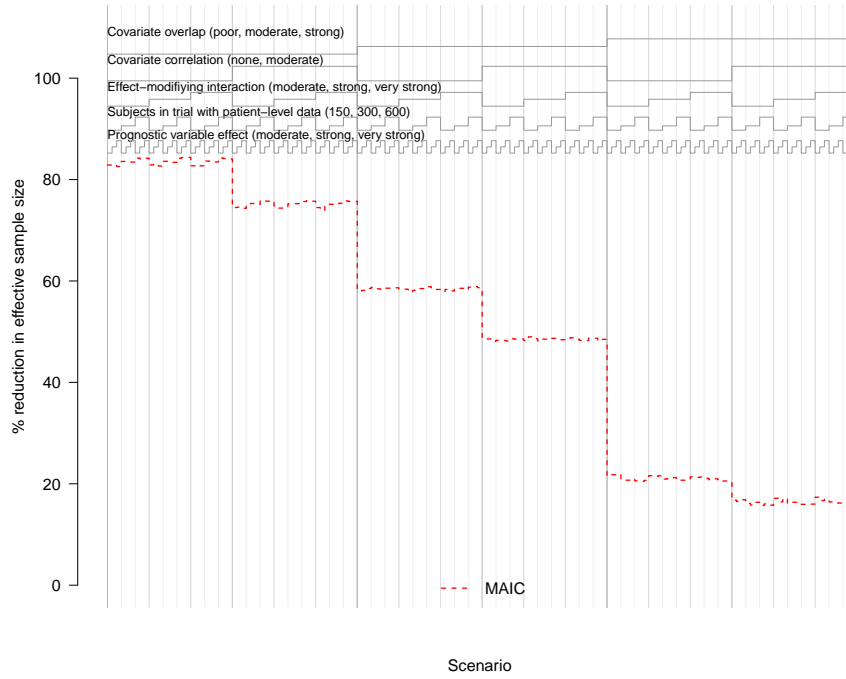

Figure 7: Mean percentage reduction in effective sample size across all simulation scenarios for matching-adjusted indirect comparison (MAIC).

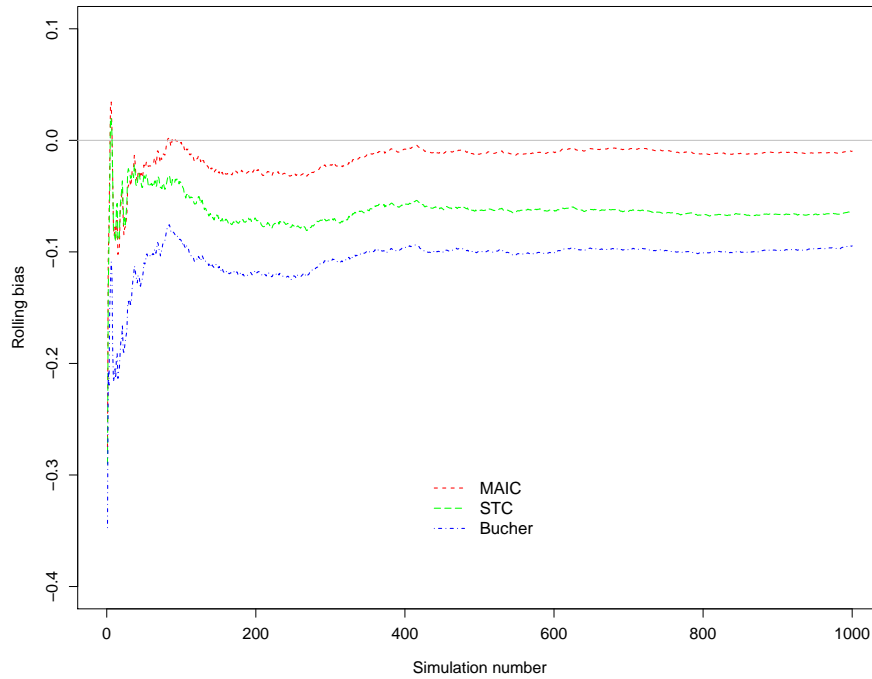

Figure 8: Bias converging over the simulations in Scenario 1. MAIC: matching-adjusted indirect comparison; STC: simulated treatment comparison.

## Appendix F: Example code

Example R code implementing MAIC, STC and the Bucher method on a simulated example is provided in this appendix. The code and data are also available at [https://github.com/remiroazocar/population\\_adjustment\\_simstudy](https://github.com/remiroazocar/population_adjustment_simstudy) in the `Example` subdirectory.

### MAIC

```
library("survival") # required for weighted Cox regression

AC.IPD <- read.csv("Example/AC_IPD.csv") # load AC patient-level data
BC.ALD <- read.csv("Example/BC_ALD.csv") # load BC aggregate-level data

N <- nrow(AC.IPD) # number of subjects in AC
X.EM <- AC.IPD[,c("X1", "X2")] # AC effect modifiers
bar.X.EM.BC <- BC.ALD[,c("mean_X1", "mean_X2")] # BC effect modifier means
K.EM <- ncol(X.EM) # number of effect modifiers

# center the AC effect modifiers on the BC means
for (k in 1:K.EM) {
  X.EM[,k] <- X.EM[,k] - bar.X.EM.BC[,k]
}

# objective function to be minimized for weight estimation
Q <- function(alpha, X.EM) {
  return(sum(exp(X.EM %*% alpha)))
}

alpha <- rep(1, K.EM) # arbitrary starting point for the optimiser
# objective function minimized using BFGS
Q.min <- optim(fn=Q, X.EM=as.matrix(X.EM), par=alpha, method="BFGS")
hat.alpha <- Q.min$par # finite solution is the logistic regression parameters
log.hat.w <- rep(0, N)
for (k in 1:K.EM) {
  log.hat.w <- log.hat.w + hat.alpha[k]*X.EM[,k]
}
hat.w <- exp(log.hat.w) # estimated weights
aess <- sum(hat.w)^2/sum(hat.w^2) # approximate effective sample size

# fit weighted Cox proportional hazards model using robust=TRUE for robust variance
outcome.fit <- coxph(Surv(time, status)~trt, robust=TRUE, weights=hat.w, data=AC.IPD)

# fitted treatment coefficient is relative effect for A vs. C
hat.Delta.AC <- summary(outcome.fit)$coef[1]
hat.var.Delta.AC <- vcov(outcome.fit)[[1]] # estimated variance for A vs. C
hat.Delta.BC <- with(BC.ALD, logHR_B) # B vs. C
hat.var.Delta.BC <- with(BC.ALD, var_logHR_B)
hat.Delta.AB <- hat.Delta.AC - hat.Delta.BC # A vs. B
hat.var.Delta.AB <- hat.var.Delta.AC + hat.var.Delta.BC
```

## STC

```
library("survival") # required for standard Cox regression

AC.IPD <- read.csv("Example/AC_IPD.csv") # load AC patient-level data
BC.ALD <- read.csv("Example/BC_ALD.csv") # load BC aggregate-level data

# fit regression of outcome on the baseline characteristics and treatment
# effect modifiers are centered at the mean BC values
# purely prognostic variables are included but not centered
outcome.fit <- coxph(Surv(time, status)~X3+X4+trt*I(X1-BC.ALD$mean_X1)+trt*I(X2-BC.ALD$mean_X2),
                    data=AC.IPD)

# estimated treatment coefficient is relative effect for A vs. C
hat.Delta.AC <- coef(outcome.fit)["trt"]
hat.var.Delta.AC <- vcov(outcome.fit)["trt", "trt"] # estimated variance for A vs. C
hat.Delta.BC <- with(BC.ALD, logHR_B) # B vs. C
hat.var.Delta.BC <- with(BC.ALD, var_logHR_B)
hat.Delta.AB <- hat.Delta.AC - hat.Delta.BC # A vs. B
hat.var.Delta.AB <- hat.var.Delta.AC + hat.var.Delta.BC
```

## Bucher method

```
library("survival") # required for standard Cox regression

AC.IPD <- read.csv("Example/AC_IPD.csv") # load AC patient-level data
BC.ALD <- read.csv("Example/BC_ALD.csv") # load BC aggregate-level data

# simple regression of outcome on treatment
outcome.fit <- coxph(Surv(time, status)~trt, data=AC.IPD)

# fitted treatment coefficient is relative effect for A vs. C
hat.Delta.AC <- coef(outcome.fit)["trt"]
hat.var.Delta.AC <- vcov(outcome.fit)["trt", "trt"] # estimated variance for A vs. C
hat.Delta.BC <- with(BC.ALD, logHR_B) # B vs. C
hat.var.Delta.BC <- with(BC.ALD, var_logHR_B)
hat.Delta.AB <- hat.Delta.AC - hat.Delta.BC # A vs. B
hat.var.Delta.AB <- hat.var.Delta.AC + hat.var.Delta.BC
```

## References

- Austin, Peter C. 2013. “The Performance of Different Propensity Score Methods for Estimating Marginal Hazard Ratios.” *Statistics in Medicine* 32 (16): 2837–49.
- Bender, Ralf, Thomas Augustin, and Maria Blettner. 2005. “Generating Survival Times to Simulate Cox Proportional Hazards Models.” *Statistics in Medicine* 24 (11): 1713–23.
- Cole, Stephen R, and Miguel A Hernán. 2008. “Constructing Inverse Probability Weights for Marginal Structural Models.” *American Journal of Epidemiology* 168 (6): 656–64.
- Cole, Stephen R, and Elizabeth A Stuart. 2010. “Generalizing Evidence from Randomized Clinical Trials to Target Populations: The Actg 320 Trial.” *American Journal of Epidemiology* 172 (1): 107–15.
- Deeks, Jonathan J, Jac Dinnes, Roberto D’Amico, Amanda J Sowden, Charlotte Sakarovich, Fujian Song, Mark Petticrew, DG Altman, and others. 2003. “Evaluating Non-Randomised Intervention Studies.” *Health Technology Assessment (Winchester, England)* 7 (27): iii–173.
- Greenland, Sander, and James M Robins. 2009. “Identifiability, Exchangeability and Confounding Revisited.” *Epidemiologic Perspectives & Innovations* 6 (1): 4.
- Hartman, Erin, Richard Grieve, Roland Ramsahai, and Jasjeet S Sekhon. 2015. “From Sample Average Treatment Effect to Population Average Treatment Effect on the Treated: Combining Experimental with Observational Studies to Estimate Population Treatment Effects.” *Journal of the Royal Statistical Society: Series A (Statistics in Society)* 178 (3): 757–78.
- Hernán, Miguel A, and James M Robins. 2006. “Estimating Causal Effects from Epidemiological Data.” *Journal of Epidemiology & Community Health* 60 (7): 578–86.
- Holland, Paul W. 1986. “Statistics and Causal Inference.” *Journal of the American Statistical Association* 81 (396): 945–60.
- Kern, Holger L, Elizabeth A Stuart, Jennifer Hill, and Donald P Green. 2016. “Assessing Methods for Generalizing Experimental Impact Estimates to Target Populations.” *Journal of Research on Educational Effectiveness* 9 (1): 103–27.
- Morris, Tim P, Ian R White, and Michael J Crowther. 2019. “Using Simulation Studies to Evaluate Statistical Methods.” *Statistics in Medicine* 38 (11): 2074–2102.
- Neyman, Jerzy S. 1923. “On the Application of Probability Theory to Agricultural Experiments. Essay on Principles. Section 9.(translated and Edited by Dm Dabrowska and Tp Speed, Statistical Science (1990), 5, 465-480).” *Annals of Agricultural Sciences* 10: 1–51.
- Phillippo, David, Tony Ades, Sofia Dias, Stephen Palmer, Keith R Abrams, and Nicky Welton. 2016. “NICE Dsu Technical Support Document 18: Methods for Population-Adjusted Indirect Comparisons in Submissions to Nice.”
- Phillippo, David M, Anthony E Ades, Sofia Dias, Stephen Palmer, Keith R Abrams, and Nicky J Welton. 2018. “Methods for Population-Adjusted Indirect Comparisons in Health Technology Appraisal.” *Medical Decision Making* 38 (2): 200–211.
- Phillippo, David M, Sofia Dias, Ahmed Elsadat, AE Ades, and Nicky J Welton. 2019. “Population Adjustment Methods for Indirect Comparisons: A Review of National Institute for Health and Care Excellence Technology Appraisals.” *International Journal of Technology Assessment in Health Care*, 1–8.
- Rosenbaum, Paul R, and Donald B Rubin. 1983. “The Central Role of the Propensity Score in Observational Studies for Causal Effects.” *Biometrika* 70 (1): 41–55.
- Rubin, Donald B. 1974. “Estimating Causal Effects of Treatments in Randomized and Nonrandomized Studies.” *Journal of Educational Psychology* 66 (5): 688.
- . 1980. “Randomization Analysis of Experimental Data: The Fisher Randomization Test Comment.” *Journal of the American Statistical Association* 75 (371): 591–93.
- . 2005. “Causal Inference Using Potential Outcomes: Design, Modeling, Decisions.” *Journal of the American Statistical Association* 100 (469): 322–31.

- Stuart, Elizabeth A, Stephen R Cole, Catherine P Bradshaw, and Philip J Leaf. 2011. “The Use of Propensity Scores to Assess the Generalizability of Results from Randomized Trials.” *Journal of the Royal Statistical Society: Series A (Statistics in Society)* 174 (2): 369–86.
- Team, R Core, and others. 2013. “R: A Language and Environment for Statistical Computing.”
- Therneau, Terry M, and Patricia M Grambsch. 2000. “The Cox Model.” In *Modeling Survival Data: Extending the Cox Model*, 39–77. Springer.
- VanderWeele, Tyler J. 2009. “Concerning the Consistency Assumption in Causal Inference.” *Epidemiology* 20 (6): 880–83.
- VanderWeele, Tyler J, and Miguel A Hernan. 2013. “Causal Inference Under Multiple Versions of Treatment.” *Journal of Causal Inference* 1 (1): 1.
